# Supplementary material for: On the nature of the anomalous event in 2021 in the dwarf nova SS Cygni and its multi-wavelength transition
Source: arXiv:2106.15756 ancillary file (2021-06-30)
Supplement: Supplementary file 1 [file si-sscyg-overall-r2.pdf]

## References

Bellm, Eric C., et al. 2019, PASP, 131, 018002
Kurita, Mikio, et al. 2020, PASJ, 72, 48
Matsubayashi, Kazuya, et al. 2019, PASJ, 71, 102

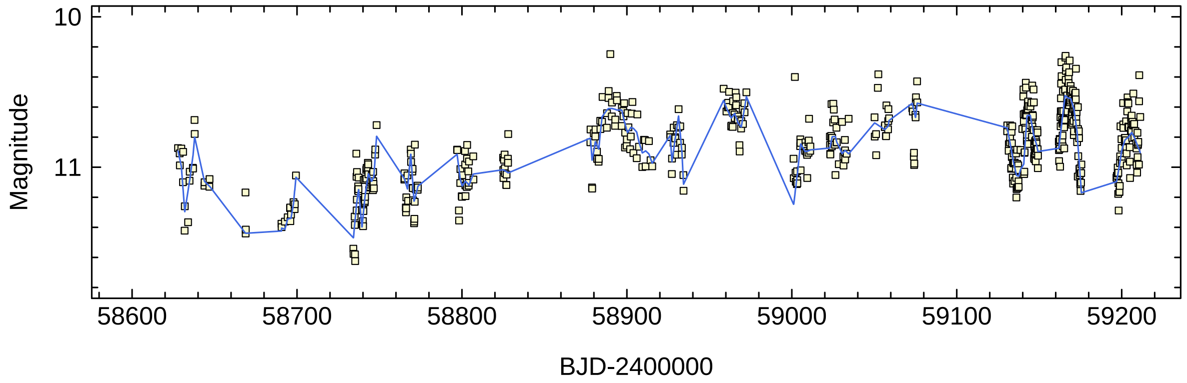


**Fig. E1.** Long-term $R_\mathrm{C}$-band light curve in SS Cyg. The squares stand for the $R_\mathrm{C}$-band photometry and the solid line represents the long-term trend which we subtract the original light curve by LOWESS in the analyses in Sec. 3.2. The data are binned to 0.1 d.

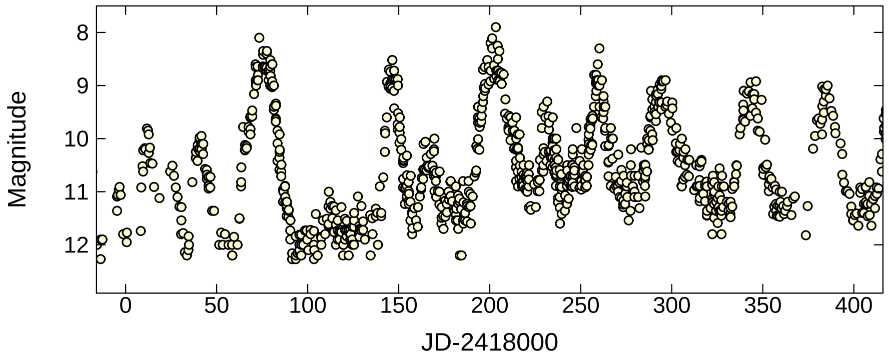


**Fig. E2.** Visual observations of SS Cyg by the AAVSO in 1908.

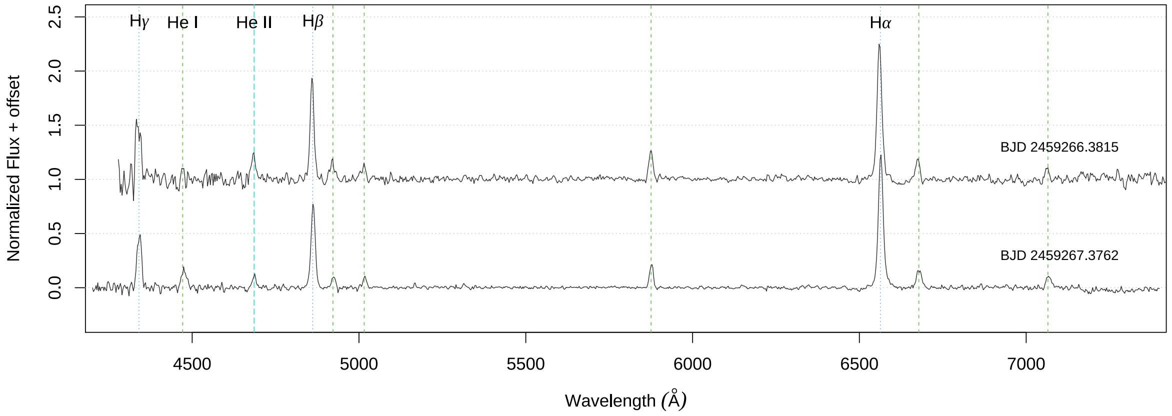


**Fig. E3.** Optical spectra during Event B taken by Kyoto Okayama Optical Low-dispersion Spectrograph with an Integral Field Unit (KOOLS-IFU; Matsubayashi et al. 2019) mounted on the 3.8-m telescope Semimei at Okayama Observatory, Kyoto University (Kurita et al. 2020). We used the VPH-blue grism whose spectral resolution is $R \sim 500$. The blue dot, green dashed, and cyan dashed lines represent the central wavelength of Balmer, He I, and He II lines, respectively.

**Table E1.** Log of observations of SS Cyg after BJD 2458700.

| Start* | End* | Mag† | Error‡ | $N$§ | Obs‖ | Band |
|---|---|---|---|---|---|---|
| 58701.7362 | 58701.7413 | 11.372 | 0.024 | 4 | HBB | $V$ |
| 58701.7371 | 58701.7422 | 11.941 | 0.034 | 4 | HBB | $B$ |
| 58703.9034 | 58703.9086 | 11.872 | 0.025 | 4 | HBB | $V$ |
| 58703.9043 | 58703.9094 | 12.478 | 0.008 | 4 | HBB | $B$ |
| 58704.8760 | 58704.8812 | 11.725 | 0.076 | 4 | HBB | $V$ |
| 58704.8769 | 58704.8820 | 12.236 | 0.128 | 4 | HBB | $B$ |
| 58717.0366 | 58717.2438 | 8.807 | 0.050 | 301 | Aka | $R_C$ |
| 58717.8489 | 58717.9227 | 9.118 | 0.071 | 50 | HBB | $V$ |
| 58717.8496 | 58717.9234 | 8.972 | 0.027 | 50 | HBB | $B$ |
| 58718.8685 | 58718.9224 | 8.770 | 0.033 | 100 | HBB | $V$ |
| 58718.8688 | 58718.9226 | 8.777 | 0.021 | 100 | HBB | $B$ |
| 58719.8641 | 58719.9092 | 8.789 | 0.022 | 40 | HBB | $V$ |
| 58719.8647 | 58719.9202 | 8.763 | 0.019 | 48 | HBB | $B$ |
| 58720.6020 | 58720.6480 | 8.915 | 0.054 | 40 | HBB | $V$ |
| 58720.6026 | 58720.6487 | 8.766 | 0.032 | 41 | HBB | $B$ |
| 58720.9610 | 58721.2435 | 8.570 | 0.022 | 383 | Aka | $R_C$ |
| 58721.9524 | 58722.2286 | 8.738 | 0.029 | 360 | Aka | $R_C$ |
| 58723.8500 | 58723.9095 | 9.202 | 0.024 | 109 | HBB | $V$ |
| 58723.8503 | 58723.9091 | 9.192 | 0.020 | 108 | HBB | $B$ |
| 58726.0186 | 58726.2602 | 9.660 | 0.041 | 50 | Aka | $R_C$ |
| 58728.1295 | 58728.2181 | 10.316 | 0.045 | 211 | Aka | $R_C$ |
| 58728.9597 | 58729.2380 | 10.475 | 0.078 | 334 | Aka | $R_C$ |
| 58730.0349 | 58730.1465 | 10.775 | 0.113 | 133 | Aka | $R_C$ |
| 58730.9764 | 58731.2520 | 10.886 | 0.102 | 460 | Aka | $R_C$ |
| 58732.2455 | 58732.2957 | 11.124 | 0.080 | 70 | Aka | $R_C$ |
| 58732.9477 | 58733.2009 | 11.518 | 0.189 | 523 | Aka | $R_C$ |
| 58734.1995 | 58734.2249 | 11.575 | 0.043 | 32 | Aka | $R_C$ |
| 58734.9512 | 58735.2157 | 11.395 | 0.109 | 163 | Aka | $R_C$ |
| 58735.9235 | 58736.2122 | 11.060 | 0.206 | 260 | Aka | $R_C$ |
| 58736.9305 | 58737.2199 | 11.282 | 0.178 | 640 | Aka | $R_C$ |
| 58739.9430 | 58740.2455 | 11.380 | 0.138 | 195 | Aka | $R_C$ |
| 58740.9381 | 58741.3013 | 11.236 | 0.129 | 525 | Aka | $R_C$ |
| 58741.9668 | 58742.2807 | 11.044 | 0.088 | 222 | Aka | $R_C$ |
| 58742.9206 | 58743.2910 | 11.006 | 0.077 | 509 | Aka | $R_C$ |
| 58743.9447 | 58744.2344 | 11.131 | 0.082 | 317 | Aka | $R_C$ |
| 58744.9380 | 58745.1856 | 11.084 | 0.074 | 333 | Aka | $R_C$ |
| 58745.9336 | 58746.3203 | 11.098 | 0.089 | 529 | Aka | $R_C$ |
| 58749.7832 | 58749.8613 | 11.412 | 0.092 | 58 | HBB | $V$ |
| 58749.7838 | 58749.8618 | 11.902 | 0.121 | 57 | HBB | $B$ |
| 58750.7614 | 58750.8617 | 11.306 | 0.137 | 100 | HBB | $V$ |
| 58750.7619 | 58750.8622 | 11.746 | 0.187 | 100 | HBB | $B$ |
| 58750.9493 | 58751.3038 | 10.899 | 0.088 | 377 | Aka | $R_C$ |
| 58751.9033 | 58752.3017 | 10.666 | 0.117 | 547 | Aka | $R_C$ |
| 58752.5143 | 58752.5742 | 10.690 | 0.082 | 60 | HBB | $V$ |
| 58752.5148 | 58752.5747 | 10.983 | 0.103 | 60 | HBB | $B$ |
| 58752.9316 | 58753.1280 | 10.165 | 0.045 | 183 | Aka | $R_C$ |
| 58753.9354 | 58754.2665 | 9.120 | 0.041 | 385 | Aka | $R_C$ |
| 58754.9487 | 58755.0193 | 8.922 | 0.015 | 98 | Aka | $R_C$ |
| 58757.0517 | 58757.2329 | 9.315 | 0.023 | 249 | Aka | $R_C$ |
| 58759.7412 | 58759.8112 | 10.343 | 0.046 | 70 | HBB | $V$ |
| 58759.7417 | 58759.8117 | 10.364 | 0.035 | 70 | HBB | $B$ |

**Table E1.** Log of observations of SS Cyg after BJD 2458700. (continued).

| Start* | End* | Mag† | Error‡ | $N$§ | Obs‖ | Band |
|---|---|---|---|---|---|---|
| 58760.2316 | 58760.2440 | 10.209 | 0.019 | 17 | Aka | $R_C$ |
| 58760.9176 | 58761.2730 | 10.259 | 0.050 | 488 | Aka | $R_C$ |
| 58761.9147 | 58761.9205 | 10.230 | 0.024 | 9 | Aka | $R_C$ |
| 58762.9011 | 58763.2909 | 10.508 | 0.113 | 512 | Aka | $R_C$ |
| 58764.9330 | 58765.2619 | 11.055 | 0.057 | 453 | Aka | $R_C$ |
| 58765.9098 | 58766.2308 | 11.273 | 0.072 | 392 | Aka | $R_C$ |
| 58766.9080 | 58766.9538 | 11.055 | 0.073 | 41 | Aka | $R_C$ |
| 58768.9476 | 58769.1972 | 10.927 | 0.081 | 332 | Aka | $R_C$ |
| 58769.9198 | 58770.1957 | 11.060 | 0.095 | 376 | Aka | $R_C$ |
| 58770.9264 | 58771.1802 | 11.357 | 0.062 | 236 | Aka | $R_C$ |
| 58771.9193 | 58771.9942 | 11.147 | 0.070 | 104 | Aka | $R_C$ |
| 58772.9125 | 58773.2453 | 11.135 | 0.068 | 457 | Aka | $R_C$ |
| 58775.9657 | 58776.1151 | 10.774 | 0.079 | 137 | Aka | $R_C$ |
| 58778.1782 | 58778.2653 | 10.745 | 0.075 | 92 | Aka | $R_C$ |
| 58778.9097 | 58779.2255 | 10.717 | 0.085 | 435 | Aka | $R_C$ |
| 58781.9306 | 58782.0405 | 10.083 | 0.031 | 152 | Aka | $R_C$ |
| 58783.0678 | 58783.1472 | 9.784 | 0.024 | 17 | Aka | $R_C$ |
| 58784.8909 | 58784.9994 | 9.546 | 0.057 | 124 | Aka | $R_C$ |
| 58785.8794 | 58786.1007 | 9.299 | 0.034 | 215 | Aka | $R_C$ |
| 58786.8793 | 58787.1959 | 9.030 | 0.011 | 436 | Aka | $R_C$ |
| 58787.8847 | 58788.1767 | 9.070 | 0.015 | 401 | Aka | $R_C$ |
| 58788.8805 | 58789.1808 | 9.128 | 0.028 | 363 | Aka | $R_C$ |
| 58790.0389 | 58790.1644 | 9.268 | 0.027 | 135 | Aka | $R_C$ |
| 58791.0394 | 58791.1104 | 9.418 | 0.028 | 28 | Aka | $R_C$ |
| 58791.8736 | 58792.1995 | 9.399 | 0.038 | 449 | Aka | $R_C$ |
| 58792.8852 | 58793.1866 | 9.652 | 0.030 | 415 | Aka | $R_C$ |
| 58793.8824 | 58794.1656 | 9.919 | 0.040 | 390 | Aka | $R_C$ |
| 58794.8698 | 58795.0366 | 10.168 | 0.050 | 133 | Aka | $R_C$ |
| 58795.8726 | 58796.1424 | 10.469 | 0.057 | 372 | Aka | $R_C$ |
| 58796.9190 | 58797.1832 | 10.881 | 0.060 | 364 | Aka | $R_C$ |
| 58798.1139 | 58798.2127 | 11.297 | 0.076 | 137 | Aka | $R_C$ |
| 58798.9348 | 58799.0439 | 11.071 | 0.101 | 142 | Aka | $R_C$ |
| 58799.8734 | 58800.1848 | 11.126 | 0.113 | 239 | Aka | $R_C$ |
| 58801.8986 | 58802.1654 | 11.086 | 0.112 | 366 | Aka | $R_C$ |
| 58802.8728 | 58803.1071 | 11.042 | 0.135 | 323 | Aka | $R_C$ |
| 58803.8719 | 58804.1302 | 11.107 | 0.058 | 356 | Aka | $R_C$ |
| 58806.8715 | 58806.9929 | 11.021 | 0.114 | 81 | Aka | $R_C$ |
| 58807.8805 | 58808.1170 | 11.169 | 0.090 | 326 | Aka | $R_C$ |
| 58808.8874 | 58809.1633 | 10.679 | 0.059 | 355 | Aka | $R_C$ |
| 58810.8886 | 58811.1133 | 10.340 | 0.064 | 310 | Aka | $R_C$ |
| 58811.8674 | 58811.9888 | 10.260 | 0.046 | 168 | Aka | $R_C$ |
| 58813.8681 | 58814.0863 | 10.436 | 0.059 | 183 | Aka | $R_C$ |
| 58815.8730 | 58816.0963 | 10.570 | 0.063 | 308 | Aka | $R_C$ |
| 58818.9917 | 58818.9946 | 10.816 | 0.031 | 5 | Aka | $R_C$ |
| 58819.8793 | 58819.9679 | 10.734 | 0.073 | 112 | Aka | $R_C$ |
| 58820.9208 | 58820.9426 | 10.941 | 0.061 | 31 | Aka | $R_C$ |
| 58821.8711 | 58822.0926 | 10.826 | 0.095 | 302 | Aka | $R_C$ |
| 58824.9117 | 58825.1002 | 10.976 | 0.100 | 211 | Aka | $R_C$ |
| 58825.8678 | 58826.0766 | 11.005 | 0.095 | 287 | Aka | $R_C$ |
| 58826.8723 | 58827.0820 | 11.087 | 0.081 | 187 | Aka | $R_C$ |
| 58827.8848 | 58828.0798 | 10.850 | 0.130 | 61 | Aka | $R_C$ |
| 58835.8811 | 58836.0696 | 9.840 | 0.031 | 260 | Aka | $R_C$ |

**Table E1.** Log of observations of SS Cyg after BJD 2458700. (continued).

| Start* | End* | Mag† | Error‡ | $N$§ | Obs‖ | Band |
|---|---|---|---|---|---|---|
| 58836.9438 | 58837.0137 | 9.602 | 0.027 | 34 | Aka | $R_C$ |
| 58840.9288 | 58841.0576 | 9.161 | 0.020 | 173 | Aka | $R_C$ |
| 58841.8936 | 58842.0606 | 9.059 | 0.018 | 120 | Aka | $R_C$ |
| 58844.8754 | 58845.0644 | 8.526 | 0.019 | 191 | Aka | $R_C$ |
| 58845.8823 | 58846.0736 | 8.412 | 0.031 | 263 | Aka | $R_C$ |
| 58848.8715 | 58849.0273 | 8.477 | 0.016 | 91 | Aka | $R_C$ |
| 58849.8926 | 58850.0607 | 8.510 | 0.024 | 204 | Aka | $R_C$ |
| 58850.8788 | 58851.0462 | 8.548 | 0.023 | 195 | Aka | $R_C$ |
| 58851.8916 | 58852.0436 | 8.534 | 0.028 | 209 | Aka | $R_C$ |
| 58852.8877 | 58853.0084 | 8.541 | 0.031 | 141 | Aka | $R_C$ |
| 58853.8808 | 58854.0357 | 8.581 | 0.030 | 215 | Aka | $R_C$ |
| 58856.8924 | 58857.0400 | 8.983 | 0.042 | 198 | Aka | $R_C$ |
| 58857.8768 | 58857.9882 | 9.205 | 0.060 | 121 | Aka | $R_C$ |
| 58858.8771 | 58859.0239 | 9.384 | 0.046 | 203 | Aka | $R_C$ |
| 58859.8730 | 58860.0026 | 9.642 | 0.041 | 179 | Aka | $R_C$ |
| 58861.8707 | 58862.0089 | 9.934 | 0.040 | 164 | Aka | $R_C$ |
| 58863.9104 | 58864.0057 | 10.096 | 0.066 | 132 | Aka | $R_C$ |
| 58864.8799 | 58864.9701 | 10.392 | 0.080 | 125 | Aka | $R_C$ |
| 58865.8730 | 58865.9006 | 10.617 | 0.090 | 39 | Aka | $R_C$ |
| 58866.8785 | 58867.0013 | 10.452 | 0.080 | 170 | Aka | $R_C$ |
| 58867.8802 | 58867.9442 | 10.620 | 0.103 | 89 | Aka | $R_C$ |
| 58868.8867 | 58868.9525 | 10.570 | 0.107 | 78 | Aka | $R_C$ |
| 58869.8801 | 58869.9972 | 10.733 | 0.077 | 162 | Aka | $R_C$ |
| 58872.8751 | 58872.9012 | 10.676 | 0.065 | 37 | Aka | $R_C$ |
| 58877.8921 | 58877.9539 | 10.760 | 0.073 | 86 | Aka | $R_C$ |
| 58878.8884 | 58878.9538 | 11.141 | 0.061 | 87 | Aka | $R_C$ |
| 58879.8921 | 58879.9197 | 10.792 | 0.105 | 39 | Aka | $R_C$ |
| 58880.8851 | 58880.9200 | 10.769 | 0.102 | 49 | Aka | $R_C$ |
| 58881.8912 | 58881.9283 | 10.933 | 0.086 | 52 | Aka | $R_C$ |
| 58882.8929 | 58882.9452 | 10.947 | 0.083 | 72 | Aka | $R_C$ |
| 58883.8893 | 58883.9649 | 10.755 | 0.186 | 105 | Aka | $R_C$ |
| 58884.9052 | 58884.9459 | 10.698 | 0.139 | 57 | Aka | $R_C$ |
| 58887.8902 | 58887.9230 | 10.670 | 0.083 | 46 | Aka | $R_C$ |
| 58888.8887 | 58888.9170 | 10.512 | 0.058 | 40 | Aka | $R_C$ |
| 58889.9022 | 58889.9487 | 10.248 | 0.141 | 8 | Aka | $R_C$ |
| 58890.8885 | 58890.9205 | 10.601 | 0.132 | 44 | Aka | $R_C$ |
| 58892.8926 | 58892.9252 | 10.693 | 0.080 | 46 | Aka | $R_C$ |
| 58893.8922 | 58893.9275 | 10.549 | 0.094 | 49 | Aka | $R_C$ |
| 58896.8951 | 58896.9256 | 10.613 | 0.174 | 36 | Aka | $R_C$ |
| 58897.8969 | 58898.3789 | 10.637 | 0.072 | 56 | Aka | $R_C$ |
| 58898.8997 | 58898.9280 | 10.773 | 0.077 | 41 | Aka | $R_C$ |
| 58899.8965 | 58900.3760 | 10.768 | 0.119 | 81 | Aka | $R_C$ |
| 58900.9108 | 58900.9290 | 10.767 | 0.196 | 25 | Aka | $R_C$ |
| 58901.9007 | 58902.3766 | 10.836 | 0.125 | 63 | Aka | $R_C$ |
| 58902.9029 | 58903.3753 | 10.602 | 0.121 | 100 | Aka | $R_C$ |
| 58903.9054 | 58903.9224 | 10.906 | 0.092 | 24 | Aka | $R_C$ |
| 58905.9084 | 58906.3731 | 10.727 | 0.146 | 101 | Aka | $R_C$ |
| 58907.3330 | 58907.3737 | 10.864 | 0.089 | 57 | Aka | $R_C$ |
| 58909.3360 | 58909.3724 | 10.999 | 0.041 | 51 | Aka | $R_C$ |
| 58910.3245 | 58910.3689 | 10.818 | 0.060 | 62 | Aka | $R_C$ |
| 58910.9057 | 58911.3688 | 10.940 | 0.119 | 80 | Aka | $R_C$ |

**Table E1.** Log of observations of SS Cyg after BJD 2458700. (continued).

| Start* | End* | Mag† | Error‡ | $N$§ | Obs‖ | Band |
|---|---|---|---|---|---|---|
| 58913.3234 | 58913.3685 | 10.827 | 0.085 | 63 | Aka | $R_C$ |
| 58914.3174 | 58914.3675 | 10.954 | 0.071 | 70 | Aka | $R_C$ |
| 58915.3523 | 58915.3588 | 10.994 | 0.079 | 10 | Aka | $R_C$ |
| 58917.3370 | 58917.3653 | 10.792 | 0.058 | 40 | Aka | $R_C$ |
| 58919.2808 | 58919.3596 | 10.413 | 0.079 | 73 | Aka | $R_C$ |
| 58920.2679 | 58920.3617 | 10.308 | 0.065 | 130 | Aka | $R_C$ |
| 58921.2795 | 58921.3464 | 10.319 | 0.073 | 90 | Aka | $R_C$ |
| 58923.2787 | 58923.3492 | 10.681 | 0.048 | 98 | Aka | $R_C$ |
| 58924.3523 | 58924.3573 | 10.743 | 0.174 | 8 | Aka | $R_C$ |
| 58926.2723 | 58926.3515 | 10.794 | 0.075 | 109 | Aka | $R_C$ |
| 58927.2780 | 58927.3536 | 10.973 | 0.082 | 105 | Aka | $R_C$ |
| 58928.2786 | 58928.3560 | 10.782 | 0.093 | 52 | Aka | $R_C$ |
| 58929.2737 | 58929.3544 | 10.806 | 0.045 | 112 | Aka | $R_C$ |
| 58930.2803 | 58930.3545 | 10.774 | 0.191 | 103 | Aka | $R_C$ |
| 58931.2653 | 58931.3533 | 10.650 | 0.122 | 121 | Aka | $R_C$ |
| 58932.2640 | 58932.3505 | 10.774 | 0.083 | 120 | Aka | $R_C$ |
| 58933.2599 | 58933.3493 | 10.891 | 0.072 | 124 | Aka | $R_C$ |
| 58934.2489 | 58934.3467 | 11.103 | 0.083 | 74 | Aka | $R_C$ |
| 58934.8922 | 58934.8976 | 11.199 | 0.047 | 4 | HBB | $V$ |
| 58934.8931 | 58934.8985 | 11.595 | 0.067 | 4 | HBB | $B$ |
| 58941.2172 | 58941.2980 | 9.013 | 0.033 | 112 | Aka | $R_C$ |
| 58942.2455 | 58942.3406 | 8.830 | 0.021 | 131 | Aka | $R_C$ |
| 58943.2468 | 58943.2698 | 8.871 | 0.076 | 30 | Aka | $R_C$ |
| 58945.2369 | 58945.3352 | 9.330 | 0.030 | 136 | Aka | $R_C$ |
| 58946.2918 | 58946.3405 | 9.636 | 0.068 | 68 | Aka | $R_C$ |
| 58947.2282 | 58947.3388 | 9.740 | 0.059 | 153 | Aka | $R_C$ |
| 58948.2516 | 58948.3360 | 9.956 | 0.046 | 117 | Aka | $R_C$ |
| 58949.1958 | 58949.3136 | 10.121 | 0.051 | 163 | Aka | $R_C$ |
| 58950.2265 | 58950.3363 | 10.145 | 0.107 | 152 | Aka | $R_C$ |
| 58953.2320 | 58953.3330 | 10.543 | 0.110 | 140 | Aka | $R_C$ |
| 58954.2203 | 58954.3294 | 10.490 | 0.093 | 151 | Aka | $R_C$ |
| 58955.2510 | 58955.3274 | 10.629 | 0.085 | 106 | Aka | $R_C$ |
| 58956.2150 | 58956.3303 | 10.516 | 0.099 | 142 | Aka | $R_C$ |
| 58960.3193 | 58960.3236 | 10.629 | 0.042 | 7 | Aka | $R_C$ |
| 58961.2369 | 58961.3278 | 10.593 | 0.077 | 126 | Aka | $R_C$ |
| 58963.2170 | 58963.3230 | 10.728 | 0.099 | 132 | Aka | $R_C$ |
| 58964.1988 | 58964.3232 | 10.626 | 0.074 | 172 | Aka | $R_C$ |
| 58965.2959 | 58965.3199 | 10.668 | 0.037 | 34 | Aka | $R_C$ |
| 58966.2129 | 58966.3213 | 10.577 | 0.061 | 150 | Aka | $R_C$ |
| 58967.2139 | 58967.3197 | 10.677 | 0.104 | 111 | Aka | $R_C$ |
| 58968.2184 | 58968.3180 | 10.861 | 0.073 | 138 | Aka | $R_C$ |
| 58969.2094 | 58969.3199 | 10.734 | 0.071 | 153 | Aka | $R_C$ |
| 58970.2156 | 58970.3189 | 10.630 | 0.085 | 143 | Aka | $R_C$ |
| 58971.2938 | 58971.3193 | 10.620 | 0.068 | 36 | Aka | $R_C$ |
| 58975.2704 | 58975.3123 | 10.715 | 0.059 | 54 | Aka | $R_C$ |
| 58976.1445 | 58976.3139 | 10.706 | 0.092 | 234 | Aka | $R_C$ |
| 58977.1897 | 58977.3003 | 10.536 | 0.137 | 146 | Aka | $R_C$ |
| 58978.2339 | 58978.3096 | 10.476 | 0.113 | 105 | Aka | $R_C$ |
| 58980.1918 | 58980.3060 | 9.939 | 0.060 | 158 | Aka | $R_C$ |
| 58981.1992 | 58981.3134 | 9.515 | 0.059 | 158 | Aka | $R_C$ |
| 58982.2295 | 58982.3117 | 9.203 | 0.035 | 114 | Aka | $R_C$ |

**Table E1.** Log of observations of SS Cyg after BJD 2458700. (continued).

| Start* | End* | Mag† | Error‡ | $N$§ | Obs‖ | Band |
|---|---|---|---|---|---|---|
| 58983.1671 | 58983.2923 | 8.940 | 0.032 | 173 | Aka | $R_C$ |
| 58984.1261 | 58984.2790 | 8.796 | 0.101 | 204 | Aka | $R_C$ |
| 58986.2086 | 58986.2676 | 9.103 | 0.025 | 14 | Aka | $R_C$ |
| 58990.1628 | 58990.2007 | 9.869 | 0.052 | 53 | Aka | $R_C$ |
| 58991.1400 | 58991.3059 | 10.161 | 0.063 | 229 | Aka | $R_C$ |
| 58991.4380 | 58991.5421 | 10.374 | 0.095 | 823 | TRT | $V$ |
| 58992.1778 | 58992.3069 | 10.037 | 0.084 | 177 | Aka | $R_C$ |
| 58992.8613 | 58992.9028 | 10.465 | 0.077 | 25 | HBB | $V$ |
| 58992.8622 | 58992.9037 | 10.696 | 0.137 | 24 | HBB | $B$ |
| 58993.1362 | 58993.3073 | 10.307 | 0.100 | 236 | Aka | $R_C$ |
| 58994.1292 | 58994.1837 | 10.386 | 0.173 | 76 | Aka | $R_C$ |
| 58996.2935 | 58996.3001 | 11.035 | 0.125 | 10 | Aka | $R_C$ |
| 58996.8416 | 58996.8724 | 11.452 | 0.090 | 19 | HBB | $V$ |
| 58996.8424 | 58996.8733 | 11.964 | 0.120 | 19 | HBB | $B$ |
| 58997.2387 | 58997.3057 | 10.880 | 0.114 | 93 | Aka | $R_C$ |
| 58997.8409 | 58997.9074 | 11.259 | 0.082 | 38 | HBB | $V$ |
| 58997.8417 | 58997.9006 | 11.740 | 0.121 | 34 | HBB | $B$ |
| 58998.0999 | 58998.3045 | 10.635 | 0.196 | 282 | Aka | $R_C$ |
| 58999.1045 | 58999.3048 | 10.869 | 0.101 | 271 | Aka | $R_C$ |
| 58999.8516 | 58999.9082 | 11.427 | 0.090 | 34 | HBB | $V$ |
| 58999.8525 | 58999.9073 | 11.972 | 0.123 | 33 | HBB | $B$ |
| 59000.8537 | 59000.8624 | 11.119 | 0.056 | 5 | HBB | $V$ |
| 59000.8546 | 59000.8633 | 11.656 | 0.089 | 6 | HBB | $B$ |
| 59001.0962 | 59001.1099 | 11.051 | 0.094 | 17 | Aka | $R_C$ |
| 59002.2975 | 59002.3062 | 11.117 | 0.116 | 13 | Aka | $R_C$ |
| 59003.0972 | 59003.3045 | 11.065 | 0.086 | 286 | Aka | $R_C$ |
| 59005.0842 | 59005.3039 | 10.849 | 0.193 | 285 | Aka | $R_C$ |
| 59008.0862 | 59008.3059 | 10.865 | 0.095 | 303 | Aka | $R_C$ |
| 59009.0734 | 59009.3039 | 10.908 | 0.100 | 317 | Aka | $R_C$ |
| 59010.0703 | 59010.2990 | 10.874 | 0.193 | 215 | Aka | $R_C$ |
| 59010.8389 | 59010.9088 | 11.509 | 0.104 | 135 | HBB | $V$ |
| 59011.1554 | 59011.2498 | 10.877 | 0.087 | 112 | Aka | $R_C$ |
| 59015.1614 | 59015.2609 | 9.047 | 0.038 | 133 | Aka | $R_C$ |
| 59016.0767 | 59016.2913 | 9.213 | 0.087 | 263 | Aka | $R_C$ |
| 59017.0832 | 59017.1828 | 9.390 | 0.148 | 115 | Aka | $R_C$ |
| 59018.0220 | 59018.0948 | 9.695 | 0.313 | 17 | Aka | $R_C$ |
| 59020.0138 | 59020.3023 | 10.229 | 0.064 | 371 | Aka | $R_C$ |
| 59021.0121 | 59021.3027 | 10.352 | 0.088 | 320 | Aka | $R_C$ |
| 59022.0036 | 59022.3061 | 10.531 | 0.145 | 326 | Aka | $R_C$ |
| 59023.0211 | 59023.3066 | 10.860 | 0.112 | 381 | Aka | $R_C$ |
| 59024.0314 | 59024.3064 | 10.782 | 0.162 | 379 | Aka | $R_C$ |
| 59025.0277 | 59025.1248 | 10.657 | 0.120 | 89 | Aka | $R_C$ |
| 59026.1013 | 59026.1406 | 10.851 | 0.139 | 43 | Aka | $R_C$ |
| 59027.0096 | 59027.2883 | 10.803 | 0.103 | 384 | Aka | $R_C$ |
| 59031.2454 | 59031.3028 | 10.935 | 0.060 | 10 | Aka | $R_C$ |
| 59032.0545 | 59032.3077 | 10.865 | 0.085 | 349 | Aka | $R_C$ |
| 59033.2335 | 59033.2532 | 10.910 | 0.046 | 18 | Aka | $R_C$ |
| 59035.0573 | 59035.0580 | 10.822 | 0.032 | 2 | Aka | $R_C$ |
| 59039.1351 | 59039.1997 | 9.068 | 0.022 | 73 | Aka | $R_C$ |
| 59040.6045 | 59040.6358 | 9.469 | 0.037 | 264 | Aka | $R_C$ |
| 59042.0644 | 59042.6292 | 9.704 | 0.066 | 135 | Aka | $R_C$ |

**Table E1.** Log of observations of SS Cyg after BJD 2458700. (continued).

| Start* | End* | Mag† | Error‡ | $N$§ | Obs‖ | Band |
|---|---|---|---|---|---|---|
| 59044.5751 | 59044.6208 | 10.253 | 0.077 | 74 | Aka | $R_{\rm C}$ |
| 59047.0039 | 59047.2341 | 10.478 | 0.088 | 134 | Aka | $R_{\rm C}$ |
| 59048.0083 | 59048.1058 | 10.822 | 0.070 | 122 | Aka | $R_{\rm C}$ |
| 59050.1345 | 59050.2065 | 10.680 | 0.087 | 98 | Aka | $R_{\rm C}$ |
| 59051.0584 | 59051.1449 | 10.900 | 0.153 | 48 | Aka | $R_{\rm C}$ |
| 59052.1621 | 59052.1882 | 10.472 | 0.109 | 37 | Aka | $R_{\rm C}$ |
| 59056.3776 | 59056.4076 | 10.730 | 0.076 | 207 | Aka | $R_{\rm C}$ |
| 59057.0337 | 59057.1306 | 10.793 | 0.110 | 118 | Aka | $R_{\rm C}$ |
| 59058.3492 | 59058.5093 | 10.708 | 0.076 | 407 | Aka | $R_{\rm C}$ |
| 59059.0917 | 59059.4094 | 10.486 | 0.062 | 28 | Aka | $R_{\rm C}$ |
| 59060.0138 | 59060.3751 | 9.975 | 0.076 | 337 | Aka | $R_{\rm C}$ |
| 59061.0101 | 59061.3748 | 9.170 | 0.048 | 427 | Aka | $R_{\rm C}$ |
| 59061.9934 | 59062.3601 | 9.010 | 0.025 | 567 | Aka | $R_{\rm C}$ |
| 59063.0103 | 59063.1703 | 9.050 | 0.028 | 142 | Aka | $R_{\rm C}$ |
| 59064.0090 | 59064.1015 | 9.209 | 0.022 | 104 | Aka | $R_{\rm C}$ |
| 59064.9972 | 59065.2648 | 9.336 | 0.046 | 423 | Aka | $R_{\rm C}$ |
| 59065.9969 | 59066.1133 | 9.298 | 0.037 | 17 | Aka | $R_{\rm C}$ |
| 59066.9922 | 59067.3144 | 9.369 | 0.045 | 45 | Aka | $R_{\rm C}$ |
| 59068.0454 | 59068.0869 | 9.498 | 0.040 | 6 | Aka | $R_{\rm C}$ |
| 59068.9910 | 59069.2034 | 9.594 | 0.058 | 21 | Aka | $R_{\rm C}$ |
| 59070.0084 | 59070.2665 | 9.896 | 0.057 | 19 | Aka | $R_{\rm C}$ |
| 59070.9954 | 59071.2353 | 10.116 | 0.062 | 14 | Aka | $R_{\rm C}$ |
| 59071.9996 | 59072.3286 | 10.393 | 0.121 | 346 | Aka | $R_{\rm C}$ |
| 59073.0247 | 59073.3711 | 10.626 | 0.067 | 149 | Aka | $R_{\rm C}$ |
| 59073.9934 | 59074.2660 | 10.956 | 0.087 | 280 | Aka | $R_{\rm C}$ |
| 59074.9788 | 59075.2408 | 10.611 | 0.115 | 271 | Aka | $R_{\rm C}$ |
| 59075.9932 | 59076.0906 | 10.559 | 0.102 | 135 | Aka | $R_{\rm C}$ |
| 59077.0027 | 59077.1285 | 10.447 | 0.091 | 174 | Aka | $R_{\rm C}$ |
| 59077.9992 | 59078.1047 | 10.159 | 0.110 | 146 | Aka | $R_{\rm C}$ |
| 59078.9663 | 59079.3770 | 9.949 | 0.100 | 601 | Aka | $R_{\rm C}$ |
| 59079.9794 | 59080.3297 | 10.006 | 0.102 | 399 | Aka | $R_{\rm C}$ |
| 59080.9784 | 59081.3351 | 10.085 | 0.076 | 440 | Aka | $R_{\rm C}$ |
| 59081.8854 | 59081.9290 | 10.100 | 0.061 | 84 | HBB | $V$ |
| 59081.9768 | 59082.3354 | 9.575 | 0.144 | 487 | Aka | $R_{\rm C}$ |
| 59082.9556 | 59083.1388 | 9.219 | 0.032 | 253 | Aka | $R_{\rm C}$ |
| 59084.3983 | 59084.4511 | 9.276 | 0.041 | 99 | Aka | $R_{\rm C}$ |
| 59084.9795 | 59085.4185 | 9.436 | 0.034 | 623 | Aka | $R_{\rm C}$ |
| 59085.9407 | 59086.3175 | 9.652 | 0.037 | 652 | Aka | $R_{\rm C}$ |
| 59086.9472 | 59087.3367 | 9.890 | 0.055 | 530 | Aka | $R_{\rm C}$ |
| 59087.6406 | 59087.7032 | 10.351 | 0.048 | 61 | HBB | $B$ |
| 59087.6411 | 59087.7037 | 10.341 | 0.050 | 61 | HBB | $V$ |
| 59087.9651 | 59088.3393 | 10.127 | 0.059 | 492 | Aka | $R_{\rm C}$ |
| 59088.9457 | 59089.3078 | 10.328 | 0.074 | 499 | Aka | $R_{\rm C}$ |
| 59089.9584 | 59090.3239 | 10.099 | 0.104 | 393 | Aka | $R_{\rm C}$ |
| 59090.9374 | 59091.3353 | 9.944 | 0.097 | 548 | Aka | $R_{\rm C}$ |
| 59091.9680 | 59092.2340 | 10.099 | 0.078 | 321 | Aka | $R_{\rm C}$ |
| 59092.9854 | 59093.2661 | 10.058 | 0.109 | 438 | Aka | $R_{\rm C}$ |
| 59093.9492 | 59094.1695 | 10.268 | 0.150 | 142 | Aka | $R_{\rm C}$ |
| 59094.9738 | 59095.3527 | 10.298 | 0.127 | 710 | Aka | $R_{\rm C}$ |
| 59095.9455 | 59096.3755 | 10.475 | 0.118 | 1209 | Aka | $R_{\rm C}$ |
| 59097.0739 | 59097.4105 | 10.650 | 0.117 | 329 | Aka | $R_{\rm C}$ |

**Table E1.** Log of observations of SS Cyg after BJD 2458700. (continued).

| Start* | End* | Mag† | Error‡ | $N$§ | Obs‖ | Band |
|---|---|---|---|---|---|---|
| 59097.7507 | 59097.8450 | 10.672 | 0.127 | 93 | HBB | $V$ |
| 59097.7512 | 59097.8456 | 10.977 | 0.173 | 93 | HBB | $B$ |
| 59097.9492 | 59098.2850 | 10.611 | 0.120 | 652 | Aka | $R_{\mathrm{C}}$ |
| 59099.2513 | 59099.3167 | 10.635 | 0.108 | 171 | Aka | $R_{\mathrm{C}}$ |
| 59099.9333 | 59100.3939 | 10.440 | 0.154 | 709 | Aka | $R_{\mathrm{C}}$ |
| 59100.9345 | 59101.3396 | 10.037 | 0.082 | 849 | Aka | $R_{\mathrm{C}}$ |
| 59102.0103 | 59102.2513 | 10.276 | 0.145 | 273 | Aka | $R_{\mathrm{C}}$ |
| 59103.3049 | 59103.3515 | 10.110 | 0.054 | 270 | Aka | $R_{\mathrm{C}}$ |
| 59104.2805 | 59104.3249 | 10.304 | 0.076 | 370 | Aka | $R_{\mathrm{C}}$ |
| 59104.9539 | 59105.0709 | 10.394 | 0.090 | 267 | Aka | $R_{\mathrm{C}}$ |
| 59105.3352 | 59105.5611 | 11.124 | 0.179 | 79 | Vih | $B$ |
| 59105.3363 | 59105.5622 | 10.800 | 0.155 | 79 | Vih | $V$ |
| 59105.3368 | 59105.5627 | 10.433 | 0.131 | 79 | Vih | $R_{\mathrm{C}}$ |
| 59105.3372 | 59105.5660 | 10.063 | 0.103 | 79 | Vih | $I_{\mathrm{C}}$ |
| 59106.2587 | 59106.5820 | 11.050 | 0.202 | 135 | Vih | $B$ |
| 59106.2596 | 59106.5734 | 10.749 | 0.156 | 130 | Vih | $V$ |
| 59106.2598 | 59106.5738 | 10.389 | 0.132 | 130 | Vih | $R_{\mathrm{C}}$ |
| 59106.2600 | 59106.5740 | 10.031 | 0.107 | 130 | Vih | $I_{\mathrm{C}}$ |
| 59107.3078 | 59107.4005 | 10.714 | 0.106 | 451 | TRT | $V$ |
| 59107.7438 | 59107.7955 | 10.705 | 0.107 | 35 | HBB | $V$ |
| 59107.7444 | 59107.7918 | 11.035 | 0.119 | 23 | HBB | $B$ |
| 59107.7482 | 59107.8065 | 10.325 | 0.142 | 35 | HBB | $R_{\mathrm{C}}$ |
| 59108.2607 | 59108.6111 | 10.371 | 0.093 | 346 | Vih | $R_{\mathrm{C}}$ |
| 59108.2992 | 59108.6106 | 10.670 | 0.106 | 310 | Vih | $V$ |
| 59108.3543 | 59108.5434 | 10.695 | 0.104 | 1372 | TRT | $V$ |
| 59109.3081 | 59109.5438 | 10.354 | 0.134 | 235 | Vih | $V$ |
| 59109.3086 | 59109.5423 | 9.996 | 0.115 | 235 | Vih | $R_{\mathrm{C}}$ |
| 59110.3549 | 59110.5998 | 10.680 | 0.093 | 245 | Vih | $V$ |
| 59110.3555 | 59110.5993 | 10.366 | 0.079 | 245 | Vih | $R_{\mathrm{C}}$ |
| 59111.2725 | 59111.5452 | 10.771 | 0.142 | 2050 | TRT | $V$ |
| 59112.3825 | 59112.4199 | 10.607 | 0.121 | 584 | TRT | $V$ |
| 59113.4166 | 59113.4885 | 10.666 | 0.089 | 567 | TRT | $V$ |
| 59114.2531 | 59114.5264 | 9.485 | 0.139 | 2225 | TRT | $V$ |
| 59118.6870 | 59118.7605 | 9.274 | 0.025 | 63 | HBB | $V$ |
| 59118.6876 | 59118.7600 | 9.213 | 0.051 | 61 | HBB | $R_{\mathrm{C}}$ |
| 59122.1039 | 59122.2575 | 9.546 | 0.051 | 519 | Ioh | $V$ |
| 59123.9996 | 59124.1858 | 9.618 | 0.050 | 94 | Ak2 | $I_{\mathrm{C}}$ |
| 59124.0007 | 59124.1850 | 10.068 | 0.051 | 94 | Ak2 | $V$ |
| 59124.7089 | 59124.7635 | 10.300 | 0.062 | 44 | HBB | $V$ |
| 59124.7095 | 59124.7640 | 10.149 | 0.050 | 42 | HBB | $R_{\mathrm{C}}$ |
| 59124.9957 | 59125.1486 | 10.351 | 0.058 | 580 | Ioh | $V$ |
| 59125.0104 | 59125.1613 | 10.374 | 0.055 | 49 | Ak2 | $V$ |
| 59125.0112 | 59125.1621 | 9.828 | 0.054 | 52 | Ak2 | $I_{\mathrm{C}}$ |
| 59125.3848 | 59125.5357 | 10.470 | 0.067 | 52 | Ak2 | $B$ |
| 59127.9164 | 59128.2219 | 11.148 | 0.123 | 320 | Ioh | $V$ |
| 59127.9737 | 59128.1265 | 11.124 | 0.114 | 59 | Ak2 | $V$ |
| 59127.9745 | 59128.1254 | 10.268 | 0.067 | 58 | Ak2 | $I_{\mathrm{C}}$ |
| 59128.3481 | 59128.5009 | 11.436 | 0.147 | 60 | Ak2 | $B$ |
| 59128.9437 | 59129.1808 | 11.396 | 0.114 | 116 | Ak2 | $V$ |
| 59128.9445 | 59129.1816 | 10.427 | 0.062 | 112 | Ak2 | $I_{\mathrm{C}}$ |
| 59129.2179 | 59129.2627 | 10.819 | 0.066 | 177 | Vih | $R_{\mathrm{C}}$ |

**Table E1.** Log of observations of SS Cyg after BJD 2458700. (continued).

| Start* | End* | Mag† | Error‡ | $N$§ | Obs‖ | Band |
|---|---|---|---|---|---|---|
| 59129.3180 | 59129.5531 | 11.755 | 0.159 | 115 | Ak2 | $B$ |
| 59132.2164 | 59132.3389 | 10.825 | 0.077 | 488 | Vih | $R_C$ |
| 59132.9562 | 59133.2742 | 10.995 | 0.095 | 183 | Aka | $R_C$ |
| 59133.9741 | 59134.1335 | 11.001 | 0.089 | 128 | Aka | $R_C$ |
| 59135.0472 | 59135.1846 | 11.025 | 0.084 | 152 | Aka | $R_C$ |
| 59135.0516 | 59135.1614 | 11.489 | 0.104 | 46 | Ak2 | $V$ |
| 59135.0524 | 59135.1622 | 10.463 | 0.077 | 49 | Ak2 | $I_C$ |
| 59135.4260 | 59135.5357 | 11.880 | 0.126 | 43 | Ak2 | $B$ |
| 59135.8951 | 59136.2798 | 11.095 | 0.129 | 430 | Aka | $R_C$ |
| 59135.9081 | 59136.1472 | 11.527 | 0.174 | 83 | Ak2 | $V$ |
| 59135.9089 | 59136.1480 | 10.498 | 0.124 | 89 | Ak2 | $I_C$ |
| 59136.2825 | 59136.5216 | 11.901 | 0.225 | 78 | Ak2 | $B$ |
| 59136.9023 | 59137.3039 | 11.051 | 0.111 | 176 | Aka | $R_C$ |
| 59136.9113 | 59136.9545 | 11.679 | 0.058 | 23 | Ak2 | $V$ |
| 59136.9121 | 59136.9553 | 10.580 | 0.046 | 23 | Ak2 | $I_C$ |
| 59137.2192 | 59137.5203 | 11.036 | 0.108 | 269 | CRI | $R_C$ |
| 59137.2206 | 59137.5200 | 10.453 | 0.070 | 269 | CRI | $I_C$ |
| 59137.2213 | 59137.5206 | 12.057 | 0.181 | 268 | CRI | $B$ |
| 59137.2220 | 59137.5208 | 11.551 | 0.133 | 536 | CRI | $V$ |
| 59137.2857 | 59137.3288 | 12.147 | 0.093 | 23 | Ak2 | $B$ |
| 59140.8827 | 59141.1350 | 10.965 | 0.108 | 318 | Aka | $R_C$ |
| 59140.8927 | 59141.1343 | 11.426 | 0.133 | 114 | Ak2 | $V$ |
| 59140.8935 | 59141.1273 | 10.447 | 0.079 | 113 | Ak2 | $I_C$ |
| 59141.2670 | 59141.5087 | 11.825 | 0.168 | 115 | Ak2 | $B$ |
| 59141.8804 | 59142.2819 | 10.613 | 0.142 | 441 | Aka | $R_C$ |
| 59142.0706 | 59142.1255 | 11.118 | 0.064 | 29 | Ak2 | $V$ |
| 59142.0715 | 59142.1263 | 10.234 | 0.051 | 29 | Ak2 | $I_C$ |
| 59142.4450 | 59142.4998 | 11.453 | 0.097 | 29 | Ak2 | $B$ |
| 59142.8922 | 59143.2640 | 10.602 | 0.123 | 512 | Aka | $R_C$ |
| 59142.9008 | 59143.1208 | 10.933 | 0.153 | 113 | Ak2 | $V$ |
| 59142.9016 | 59143.1216 | 10.145 | 0.101 | 113 | Ak2 | $I_C$ |
| 59143.2751 | 59143.4951 | 11.199 | 0.205 | 113 | Ak2 | $B$ |
| 59145.8823 | 59146.0624 | 11.039 | 0.141 | 92 | Ak2 | $V$ |
| 59145.8831 | 59146.0672 | 10.193 | 0.100 | 94 | Ak2 | $I_C$ |
| 59145.8841 | 59146.1097 | 10.665 | 0.121 | 272 | Aka | $R_C$ |
| 59146.2567 | 59146.4387 | 11.361 | 0.185 | 93 | Ak2 | $B$ |
| 59146.8900 | 59148.0999 | 10.890 | 0.099 | 1687 | Aka | $R_C$ |
| 59146.8940 | 59147.1356 | 10.361 | 0.072 | 118 | Ak2 | $I_C$ |
| 59147.2498 | 59147.3766 | 10.344 | 0.054 | 112 | CRI | $I_C$ |
| 59147.2500 | 59147.3757 | 10.889 | 0.080 | 111 | CRI | $R_C$ |
| 59147.2503 | 59147.3771 | 11.855 | 0.138 | 112 | CRI | $B$ |
| 59147.2675 | 59147.5091 | 11.673 | 0.161 | 120 | Ak2 | $B$ |
| 59147.8872 | 59148.0466 | 10.322 | 0.072 | 78 | Ak2 | $I_C$ |
| 59148.2409 | 59148.3167 | 10.290 | 0.055 | 69 | CRI | $I_C$ |
| 59148.2411 | 59148.3170 | 10.812 | 0.091 | 69 | CRI | $R_C$ |
| 59148.2414 | 59148.3161 | 11.782 | 0.151 | 68 | CRI | $B$ |
| 59148.2608 | 59148.4202 | 11.653 | 0.152 | 78 | Ak2 | $B$ |
| 59148.8802 | 59149.2392 | 10.881 | 0.123 | 473 | Aka | $R_C$ |
| 59148.8874 | 59149.1686 | 10.325 | 0.089 | 143 | Ak2 | $I_C$ |
| 59149.2609 | 59149.5342 | 11.682 | 0.192 | 128 | Ak2 | $B$ |
| 59149.8891 | 59150.2389 | 10.624 | 0.138 | 475 | Aka | $R_C$ |

**Table E1.** Log of observations of SS Cyg after BJD 2458700. (continued).

| Start* | End* | Mag† | Error‡ | $N$§ | Obs‖ | Band |
|---|---|---|---|---|---|---|
| 59149.8975 | 59150.1255 | 10.192 | 0.065 | 117 | Ak2 | $I_C$ |
| 59150.2710 | 59150.4990 | 11.522 | 0.142 | 115 | Ak2 | $B$ |
| 59150.9897 | 59151.2508 | 9.787 | 0.139 | 346 | Aka | $R_C$ |
| 59150.9988 | 59151.1838 | 9.569 | 0.081 | 92 | Ak2 | $I_C$ |
| 59151.3723 | 59151.5534 | 10.162 | 0.148 | 88 | Ak2 | $B$ |
| 59151.8890 | 59151.9897 | 9.243 | 0.029 | 95 | Aka | $R_C$ |
| 59151.8976 | 59151.9900 | 9.067 | 0.044 | 33 | Ak2 | $I_C$ |
| 59152.2712 | 59152.3636 | 9.263 | 0.031 | 36 | Ak2 | $B$ |
| 59152.8877 | 59154.2002 | 9.134 | 0.033 | 1112 | Aka | $R_C$ |
| 59152.9208 | 59153.1084 | 8.976 | 0.025 | 68 | Ak2 | $I_C$ |
| 59153.2944 | 59153.4465 | 9.168 | 0.027 | 51 | Ak2 | $B$ |
| 59153.8860 | 59154.0945 | 8.973 | 0.023 | 98 | Ak2 | $I_C$ |
| 59154.2596 | 59154.4720 | 9.162 | 0.029 | 102 | Ak2 | $B$ |
| 59154.5533 | 59154.6217 | 9.252 | 0.050 | 89 | HBB | $V$ |
| 59154.5537 | 59154.6221 | 9.214 | 0.074 | 88 | HBB | $R_C$ |
| 59154.8853 | 59154.9288 | 9.186 | 0.065 | 15 | Aka | $R_C$ |
| 59156.8686 | 59157.1761 | 9.557 | 0.041 | 219 | Aka | $R_C$ |
| 59156.8806 | 59157.1513 | 9.310 | 0.039 | 68 | Ak2 | $I_C$ |
| 59157.2541 | 59157.5248 | 9.674 | 0.042 | 68 | Ak2 | $B$ |
| 59157.8764 | 59158.2514 | 9.770 | 0.057 | 510 | Aka | $R_C$ |
| 59157.8819 | 59158.1001 | 9.469 | 0.042 | 112 | Ak2 | $I_C$ |
| 59158.2554 | 59158.4736 | 9.936 | 0.049 | 111 | Ak2 | $B$ |
| 59158.8826 | 59158.9811 | 9.960 | 0.050 | 65 | Aka | $R_C$ |
| 59158.8888 | 59158.9262 | 9.647 | 0.061 | 20 | Ak2 | $I_C$ |
| 59159.1980 | 59159.3557 | 9.655 | 0.063 | 142 | CRI | $I_C$ |
| 59159.1983 | 59159.3560 | 9.893 | 0.073 | 142 | CRI | $R_C$ |
| 59159.1986 | 59159.3551 | 10.372 | 0.082 | 140 | CRI | $B$ |
| 59159.2623 | 59159.3016 | 10.223 | 0.048 | 21 | Ak2 | $B$ |
| 59160.4089 | 59160.4537 | 10.329 | 0.065 | 130 | Aka | $R_C$ |
| 59161.2128 | 59162.1637 | 10.718 | 0.173 | 1003 | Aka | $R_C$ |
| 59161.8767 | 59162.1064 | 10.393 | 0.070 | 117 | Ak2 | $I_C$ |
| 59162.2503 | 59162.4819 | 11.605 | 0.174 | 118 | Ak2 | $B$ |
| 59162.8747 | 59163.2089 | 10.630 | 0.124 | 459 | Aka | $R_C$ |
| 59162.8811 | 59163.1644 | 10.144 | 0.101 | 144 | Ak2 | $I_C$ |
| 59163.2547 | 59163.5380 | 11.301 | 0.192 | 145 | Ak2 | $B$ |
| 59163.8767 | 59164.2118 | 10.774 | 0.108 | 462 | Aka | $R_C$ |
| 59163.8769 | 59164.1736 | 10.262 | 0.087 | 152 | Ak2 | $I_C$ |
| 59164.2426 | 59164.5472 | 11.470 | 0.178 | 152 | Ak2 | $B$ |
| 59164.9244 | 59165.2165 | 10.767 | 0.132 | 400 | Aka | $R_C$ |
| 59164.9345 | 59165.1492 | 10.258 | 0.091 | 110 | Ak2 | $I_C$ |
| 59165.3080 | 59165.5227 | 11.429 | 0.239 | 108 | Ak2 | $B$ |
| 59165.8762 | 59166.1872 | 10.340 | 0.116 | 427 | Aka | $R_C$ |
| 59165.8954 | 59166.1065 | 9.896 | 0.094 | 108 | Ak2 | $I_C$ |
| 59166.2689 | 59166.4800 | 10.941 | 0.196 | 108 | Ak2 | $B$ |
| 59166.8770 | 59167.1910 | 10.566 | 0.101 | 427 | Aka | $R_C$ |
| 59166.8881 | 59167.1676 | 10.947 | 0.124 | 140 | Ak2 | $V$ |
| 59166.8889 | 59167.1683 | 10.074 | 0.080 | 141 | Ak2 | $I_C$ |
| 59167.2625 | 59167.5282 | 11.283 | 0.168 | 125 | Ak2 | $B$ |
| 59167.8726 | 59168.1816 | 10.511 | 0.152 | 424 | Aka | $R_C$ |
| 59167.8805 | 59168.1465 | 10.905 | 0.171 | 136 | Ak2 | $V$ |
| 59167.8813 | 59168.1473 | 10.053 | 0.105 | 137 | Ak2 | $I_C$ |

**Table E1.** Log of observations of SS Cyg after BJD 2458700. (continued).

| Start* | End* | Mag† | Error‡ | $N$§ | Obs‖ | Band |
|---|---|---|---|---|---|---|
| 59168.2549 | 59168.5228 | 11.258 | 0.211 | 136 | Ak2 | $B$ |
| 59168.8667 | 59169.1450 | 10.501 | 0.126 | 381 | Aka | $R_C$ |
| 59168.8669 | 59169.1544 | 10.848 | 0.142 | 146 | Ak2 | $V$ |
| 59168.8677 | 59169.1533 | 10.028 | 0.091 | 145 | Ak2 | $I_C$ |
| 59169.2413 | 59169.5249 | 11.178 | 0.178 | 143 | Ak2 | $B$ |
| 59169.8815 | 59170.1333 | 10.609 | 0.103 | 293 | Aka | $R_C$ |
| 59169.8887 | 59170.1303 | 10.968 | 0.128 | 101 | Ak2 | $V$ |
| 59169.8895 | 59170.1311 | 10.122 | 0.092 | 104 | Ak2 | $I_C$ |
| 59170.2630 | 59170.4850 | 11.318 | 0.153 | 91 | Ak2 | $B$ |
| 59170.8632 | 59171.0778 | 10.761 | 0.107 | 261 | Aka | $R_C$ |
| 59170.8815 | 59171.1176 | 11.146 | 0.138 | 76 | Ak2 | $V$ |
| 59170.8823 | 59171.1184 | 10.207 | 0.092 | 94 | Ak2 | $I_C$ |
| 59171.2558 | 59171.4920 | 11.536 | 0.165 | 89 | Ak2 | $B$ |
| 59171.5880 | 59171.6945 | 10.955 | 0.140 | 99 | HBB | $V$ |
| 59171.5885 | 59171.6951 | 10.513 | 0.116 | 99 | HBB | $R_C$ |
| 59171.9412 | 59172.1321 | 10.547 | 0.115 | 203 | Aka | $R_C$ |
| 59171.9560 | 59172.1311 | 10.871 | 0.154 | 61 | Ak2 | $V$ |
| 59171.9568 | 59172.1300 | 10.033 | 0.107 | 65 | Ak2 | $I_C$ |
| 59172.3303 | 59172.5055 | 11.231 | 0.174 | 59 | Ak2 | $B$ |
| 59172.9020 | 59172.9027 | 10.834 | 0.080 | 2 | Aka | $R_C$ |
| 59174.0102 | 59175.1055 | 11.025 | 0.164 | 669 | Aka | $R_C$ |
| 59174.8828 | 59175.1166 | 11.609 | 0.089 | 114 | Ak2 | $V$ |
| 59174.8836 | 59175.1174 | 10.542 | 0.061 | 116 | Ak2 | $I_C$ |
| 59175.2571 | 59175.4890 | 12.028 | 0.128 | 114 | Ak2 | $B$ |
| 59176.8598 | 59177.1345 | 10.936 | 0.097 | 371 | Aka | $R_C$ |
| 59176.8627 | 59177.1295 | 11.393 | 0.110 | 135 | Ak2 | $V$ |
| 59176.8635 | 59177.1303 | 10.361 | 0.081 | 136 | Ak2 | $I_C$ |
| 59177.2371 | 59177.5039 | 11.804 | 0.157 | 133 | Ak2 | $B$ |
| 59177.8762 | 59178.1342 | 10.722 | 0.106 | 238 | Aka | $R_C$ |
| 59177.8872 | 59178.0967 | 11.192 | 0.103 | 62 | Ak2 | $V$ |
| 59177.8880 | 59178.0975 | 10.228 | 0.065 | 61 | Ak2 | $I_C$ |
| 59178.2616 | 59178.4710 | 11.634 | 0.151 | 60 | Ak2 | $B$ |
| 59178.8682 | 59179.1383 | 10.526 | 0.064 | 222 | Aka | $R_C$ |
| 59178.8802 | 59178.9215 | 10.914 | 0.082 | 21 | Ak2 | $V$ |
| 59178.8810 | 59179.1355 | 10.020 | 0.058 | 69 | Ak2 | $I_C$ |
| 59179.2545 | 59179.4835 | 11.306 | 0.109 | 55 | Ak2 | $B$ |
| 59179.9667 | 59180.2347 | 9.307 | 0.070 | 327 | Aka | $R_C$ |
| 59179.9951 | 59180.0952 | 9.405 | 0.025 | 56 | Ak2 | $V$ |
| 59179.9959 | 59180.0940 | 9.181 | 0.022 | 51 | Ak2 | $I_C$ |
| 59180.3694 | 59180.4695 | 9.470 | 0.030 | 52 | Ak2 | $B$ |
| 59180.8999 | 59181.2106 | 8.901 | 0.044 | 131 | Aka | $R_C$ |
| 59181.8599 | 59182.0169 | 8.906 | 0.027 | 216 | Aka | $R_C$ |
| 59181.8694 | 59182.0157 | 8.945 | 0.025 | 75 | Ak2 | $V$ |
| 59181.8702 | 59182.0165 | 8.770 | 0.025 | 74 | Ak2 | $I_C$ |
| 59182.2437 | 59182.3921 | 8.938 | 0.030 | 76 | Ak2 | $B$ |
| 59182.8572 | 59183.1486 | 9.027 | 0.035 | 391 | Aka | $R_C$ |
| 59182.8615 | 59182.9324 | 9.072 | 0.026 | 34 | Ak2 | $V$ |
| 59182.8623 | 59182.9332 | 8.867 | 0.031 | 32 | Ak2 | $I_C$ |
| 59183.2359 | 59183.3067 | 9.062 | 0.030 | 34 | Ak2 | $B$ |
| 59183.8810 | 59184.2152 | 9.134 | 0.031 | 355 | Aka | $R_C$ |
| 59183.8929 | 59183.9341 | 8.952 | 0.032 | 22 | Ak2 | $I_C$ |

**Table E1.** Log of observations of SS Cyg after BJD 2458700. (continued).

| Start* | End* | Mag† | Error‡ | $N$§ | Obs‖ | Band |
|---|---|---|---|---|---|---|
| 59183.8941 | 59183.9333 | 9.197 | 0.026 | 21 | Ak2 | $V$ |
| 59184.2664 | 59184.3077 | 9.198 | 0.036 | 22 | Ak2 | $B$ |
| 59184.8769 | 59185.0872 | 9.256 | 0.042 | 246 | Aka | $R_C$ |
| 59184.8823 | 59184.9631 | 9.320 | 0.018 | 36 | Ak2 | $V$ |
| 59184.8831 | 59184.9639 | 9.033 | 0.028 | 36 | Ak2 | $I_C$ |
| 59185.2567 | 59185.3374 | 9.345 | 0.023 | 36 | Ak2 | $B$ |
| 59185.8732 | 59186.1448 | 9.388 | 0.040 | 370 | Aka | $R_C$ |
| 59185.8818 | 59185.9327 | 9.489 | 0.039 | 26 | Ak2 | $V$ |
| 59185.8826 | 59185.9335 | 9.165 | 0.038 | 26 | Ak2 | $I_C$ |
| 59186.2561 | 59186.3071 | 9.531 | 0.043 | 26 | Ak2 | $B$ |
| 59186.8724 | 59187.1111 | 9.497 | 0.045 | 320 | Aka | $R_C$ |
| 59186.8802 | 59186.9077 | 9.588 | 0.020 | 14 | Ak2 | $V$ |
| 59186.8810 | 59186.9085 | 9.241 | 0.024 | 15 | Ak2 | $I_C$ |
| 59187.2545 | 59187.2840 | 9.641 | 0.027 | 16 | Ak2 | $B$ |
| 59187.8604 | 59188.1421 | 9.592 | 0.058 | 356 | Aka | $R_C$ |
| 59187.8673 | 59187.9283 | 9.702 | 0.041 | 32 | Ak2 | $V$ |
| 59187.8681 | 59187.9291 | 9.346 | 0.033 | 32 | Ak2 | $I_C$ |
| 59188.2416 | 59188.3026 | 9.762 | 0.043 | 32 | Ak2 | $B$ |
| 59188.8632 | 59189.1113 | 9.782 | 0.047 | 341 | Aka | $R_C$ |
| 59188.8686 | 59188.9078 | 9.935 | 0.033 | 21 | Ak2 | $V$ |
| 59188.8694 | 59188.9086 | 9.524 | 0.039 | 21 | Ak2 | $I_C$ |
| 59189.2429 | 59189.2821 | 10.000 | 0.034 | 21 | Ak2 | $B$ |
| 59189.8610 | 59190.1302 | 10.061 | 0.070 | 369 | Aka | $R_C$ |
| 59189.8644 | 59189.9115 | 10.220 | 0.059 | 25 | Ak2 | $V$ |
| 59189.8652 | 59189.9123 | 9.719 | 0.059 | 25 | Ak2 | $I_C$ |
| 59190.2387 | 59190.2858 | 10.308 | 0.071 | 25 | Ak2 | $B$ |
| 59190.9557 | 59191.1055 | 10.309 | 0.078 | 164 | Aka | $R_C$ |
| 59190.9610 | 59190.9925 | 9.884 | 0.039 | 15 | Ak2 | $I_C$ |
| 59190.9681 | 59190.9917 | 10.503 | 0.038 | 13 | Ak2 | $V$ |
| 59191.3424 | 59191.3661 | 10.651 | 0.070 | 13 | Ak2 | $B$ |
| 59191.8615 | 59192.1280 | 10.617 | 0.068 | 335 | Aka | $R_C$ |
| 59191.8678 | 59191.9171 | 10.860 | 0.047 | 26 | Ak2 | $V$ |
| 59191.8686 | 59191.9178 | 10.169 | 0.041 | 26 | Ak2 | $I_C$ |
| 59192.2422 | 59192.2914 | 11.053 | 0.072 | 26 | Ak2 | $B$ |
| 59192.8685 | 59193.1255 | 10.697 | 0.115 | 353 | Aka | $R_C$ |
| 59192.8745 | 59192.9117 | 10.848 | 0.109 | 20 | Ak2 | $V$ |
| 59192.8753 | 59192.9125 | 10.106 | 0.069 | 20 | Ak2 | $I_C$ |
| 59193.2489 | 59193.2861 | 11.078 | 0.135 | 20 | Ak2 | $B$ |
| 59194.0105 | 59194.0623 | 11.013 | 0.083 | 69 | Aka | $R_C$ |
| 59194.8587 | 59195.0265 | 10.661 | 0.133 | 134 | Aka | $R_C$ |
| 59194.8639 | 59194.9110 | 10.932 | 0.141 | 25 | Ak2 | $V$ |
| 59194.8647 | 59194.9118 | 10.156 | 0.090 | 25 | Ak2 | $I_C$ |
| 59195.2383 | 59195.2853 | 11.188 | 0.183 | 25 | Ak2 | $B$ |
| 59195.8670 | 59196.0881 | 10.793 | 0.105 | 252 | Aka | $R_C$ |
| 59195.8776 | 59195.9287 | 10.247 | 0.055 | 15 | Ak2 | $I_C$ |
| 59195.8827 | 59195.9279 | 11.025 | 0.114 | 14 | Ak2 | $V$ |
| 59196.2570 | 59196.3022 | 11.306 | 0.189 | 12 | Ak2 | $B$ |
| 59196.8642 | 59197.0510 | 11.067 | 0.062 | 257 | Aka | $R_C$ |
| 59196.8728 | 59196.9100 | 11.526 | 0.083 | 20 | Ak2 | $V$ |
| 59196.8736 | 59196.9108 | 10.472 | 0.058 | 20 | Ak2 | $I_C$ |
| 59197.2471 | 59197.2843 | 11.970 | 0.141 | 20 | Ak2 | $B$ |

**Table E1.** Log of observations of SS Cyg after BJD 2458700. (continued).

| Start* | End* | Mag† | Error‡ | $N$§ | Obs‖ | Band |
|---|---|---|---|---|---|---|
| 59197.8837 | 59198.0881 | 11.077 | 0.110 | 266 | Aka | $R_C$ |
| 59197.8948 | 59197.9027 | 11.653 | 0.036 | 5 | Ak2 | $V$ |
| 59197.8956 | 59197.9054 | 10.605 | 0.030 | 5 | Ak2 | $I_C$ |
| 59198.2692 | 59198.2770 | 12.104 | 0.046 | 5 | Ak2 | $B$ |
| 59198.8680 | 59199.0658 | 10.982 | 0.105 | 272 | Aka | $R_C$ |
| 59198.8713 | 59198.8851 | 11.574 | 0.093 | 8 | Ak2 | $V$ |
| 59198.8721 | 59198.8859 | 10.528 | 0.038 | 8 | Ak2 | $I_C$ |
| 59199.2456 | 59199.2594 | 11.981 | 0.108 | 8 | Ak2 | $B$ |
| 59199.8853 | 59200.1118 | 10.909 | 0.093 | 311 | Aka | $R_C$ |
| 59199.8927 | 59199.9044 | 11.215 | 0.109 | 7 | Ak2 | $V$ |
| 59199.8935 | 59199.9052 | 10.305 | 0.068 | 7 | Ak2 | $I_C$ |
| 59200.2670 | 59200.2787 | 11.516 | 0.140 | 7 | Ak2 | $B$ |
| 59200.8934 | 59201.0627 | 10.718 | 0.128 | 233 | Aka | $R_C$ |
| 59200.8956 | 59200.9133 | 11.011 | 0.097 | 10 | Ak2 | $V$ |
| 59200.8964 | 59200.9141 | 10.120 | 0.065 | 10 | Ak2 | $I_C$ |
| 59201.2699 | 59201.2876 | 11.314 | 0.111 | 10 | Ak2 | $B$ |
| 59201.8890 | 59202.0898 | 10.819 | 0.108 | 266 | Aka | $R_C$ |
| 59201.8928 | 59201.9065 | 11.176 | 0.083 | 8 | Ak2 | $V$ |
| 59201.8975 | 59201.9073 | 10.233 | 0.049 | 6 | Ak2 | $I_C$ |
| 59202.2691 | 59202.2808 | 11.491 | 0.071 | 7 | Ak2 | $B$ |
| 59202.8978 | 59203.0744 | 10.943 | 0.094 | 235 | Aka | $R_C$ |
| 59202.9016 | 59202.9252 | 11.381 | 0.060 | 13 | Ak2 | $V$ |
| 59202.9064 | 59202.9261 | 10.373 | 0.036 | 11 | Ak2 | $I_C$ |
| 59203.2760 | 59203.2996 | 11.734 | 0.091 | 13 | Ak2 | $B$ |
| 59203.8613 | 59204.0935 | 10.641 | 0.137 | 319 | Aka | $R_C$ |
| 59203.8656 | 59203.9165 | 11.012 | 0.105 | 27 | Ak2 | $V$ |
| 59203.8664 | 59203.9173 | 10.136 | 0.073 | 27 | Ak2 | $I_C$ |
| 59204.2399 | 59204.2908 | 11.310 | 0.135 | 27 | Ak2 | $B$ |
| 59204.8899 | 59205.0529 | 10.988 | 0.124 | 211 | Aka | $R_C$ |
| 59204.8917 | 59204.9113 | 11.256 | 0.068 | 11 | Ak2 | $V$ |
| 59204.8925 | 59204.9121 | 10.334 | 0.052 | 11 | Ak2 | $I_C$ |
| 59205.2660 | 59205.2856 | 11.602 | 0.073 | 11 | Ak2 | $B$ |
| 59205.8755 | 59206.0784 | 10.695 | 0.109 | 188 | Aka | $R_C$ |
| 59206.8778 | 59207.0114 | 10.701 | 0.107 | 184 | Aka | $R_C$ |
| 59206.8817 | 59206.8896 | 11.069 | 0.149 | 5 | Ak2 | $V$ |
| 59206.8825 | 59206.8904 | 10.156 | 0.110 | 5 | Ak2 | $I_C$ |
| 59207.2560 | 59207.2639 | 11.405 | 0.160 | 5 | Ak2 | $B$ |
| 59208.8634 | 59209.0927 | 10.914 | 0.105 | 315 | Aka | $R_C$ |
| 59208.8675 | 59208.8793 | 11.337 | 0.071 | 6 | Ak2 | $V$ |
| 59208.8683 | 59208.8820 | 10.310 | 0.081 | 7 | Ak2 | $I_C$ |
| 59209.2418 | 59209.2555 | 11.772 | 0.093 | 7 | Ak2 | $B$ |
| 59209.8637 | 59210.0774 | 10.841 | 0.098 | 275 | Aka | $R_C$ |
| 59209.8671 | 59209.8828 | 11.304 | 0.157 | 9 | Ak2 | $V$ |
| 59209.8679 | 59209.8836 | 10.279 | 0.104 | 9 | Ak2 | $I_C$ |
| 59210.2414 | 59210.2571 | 11.720 | 0.229 | 9 | Ak2 | $B$ |
| 59211.8691 | 59212.0697 | 9.492 | 0.115 | 273 | Aka | $R_C$ |
| 59211.8721 | 59211.8937 | 9.724 | 0.026 | 12 | Ak2 | $V$ |
| 59211.8729 | 59211.8944 | 9.383 | 0.028 | 12 | Ak2 | $I_C$ |
| 59212.2464 | 59212.2680 | 9.849 | 0.037 | 12 | Ak2 | $B$ |
| 59212.9097 | 59212.9257 | 9.087 | 0.047 | 19 | Aka | $R_C$ |
| 59213.8671 | 59214.0738 | 8.973 | 0.033 | 284 | Aka | $R_C$ |

**Table E1.** Log of observations of SS Cyg after BJD 2458700. (continued).

| Start* | End* | Mag† | Error‡ | $N$§ | Obs‖ | Band |
|---|---|---|---|---|---|---|
| 59213.8704 | 59213.8822 | 8.987 | 0.012 | 7 | Ak2 | $B$ |
| 59213.8711 | 59213.8828 | 8.999 | 0.017 | 7 | Ak2 | $V$ |
| 59213.8719 | 59213.8836 | 8.831 | 0.013 | 7 | Ak2 | $I_C$ |
| 59214.8734 | 59215.0705 | 9.057 | 0.026 | 271 | Aka | $R_C$ |
| 59214.8775 | 59214.8971 | 9.095 | 0.018 | 11 | Ak2 | $B$ |
| 59214.8782 | 59214.8978 | 9.092 | 0.014 | 11 | Ak2 | $V$ |
| 59214.8790 | 59214.8966 | 8.896 | 0.019 | 10 | Ak2 | $I_C$ |
| 59215.8756 | 59216.0733 | 8.966 | 0.058 | 272 | Aka | $R_C$ |
| 59215.8782 | 59215.8919 | 9.082 | 0.017 | 8 | Ak2 | $B$ |
| 59215.8789 | 59215.8926 | 9.055 | 0.018 | 8 | Ak2 | $V$ |
| 59215.8797 | 59215.8934 | 8.813 | 0.013 | 8 | Ak2 | $I_C$ |
| 59216.8643 | 59216.8858 | 9.082 | 0.012 | 12 | Ak2 | $B$ |
| 59216.8649 | 59216.8865 | 9.061 | 0.013 | 12 | Ak2 | $V$ |
| 59216.8657 | 59216.8873 | 8.826 | 0.019 | 12 | Ak2 | $I_C$ |
| 59216.8667 | 59216.9746 | 9.001 | 0.035 | 144 | Aka | $R_C$ |
| 59217.8741 | 59217.8898 | 9.022 | 0.030 | 9 | Ak2 | $B$ |
| 59217.8747 | 59217.8924 | 9.006 | 0.019 | 10 | Ak2 | $V$ |
| 59217.8755 | 59217.8932 | 8.794 | 0.029 | 10 | Ak2 | $I_C$ |
| 59217.8760 | 59217.9972 | 8.954 | 0.047 | 85 | Aka | $R_C$ |
| 59218.8714 | 59219.0443 | 8.710 | 0.061 | 237 | Aka | $R_C$ |
| 59218.8743 | 59218.8939 | 8.740 | 0.033 | 11 | Ak2 | $B$ |
| 59218.8750 | 59218.8946 | 8.712 | 0.026 | 11 | Ak2 | $V$ |
| 59218.8758 | 59218.8954 | 8.514 | 0.031 | 11 | Ak2 | $I_C$ |
| 59219.9247 | 59220.0159 | 8.649 | 0.041 | 125 | Aka | $R_C$ |
| 59219.9284 | 59219.9421 | 8.641 | 0.015 | 8 | Ak2 | $B$ |
| 59219.9290 | 59219.9427 | 8.642 | 0.018 | 7 | Ak2 | $V$ |
| 59219.9298 | 59219.9337 | 8.456 | 0.037 | 3 | Ak2 | $I_C$ |
| 59220.8740 | 59220.9689 | 8.589 | 0.027 | 121 | Aka | $R_C$ |
| 59220.8786 | 59220.8923 | 8.575 | 0.032 | 8 | Ak2 | $B$ |
| 59220.8792 | 59220.8929 | 8.575 | 0.025 | 8 | Ak2 | $V$ |
| 59220.8859 | 59220.8937 | 8.430 | 0.020 | 5 | Ak2 | $I_C$ |
| 59221.8851 | 59222.0477 | 8.570 | 0.033 | 192 | Aka | $R_C$ |
| 59221.9003 | 59221.9199 | 8.560 | 0.029 | 11 | Ak2 | $B$ |
| 59221.9009 | 59221.9205 | 8.584 | 0.020 | 11 | Ak2 | $V$ |
| 59221.9017 | 59221.9213 | 8.410 | 0.026 | 11 | Ak2 | $I_C$ |
| 59222.8836 | 59222.9150 | 8.637 | 0.039 | 16 | Ak2 | $B$ |
| 59222.8842 | 59222.9156 | 8.656 | 0.036 | 17 | Ak2 | $V$ |
| 59222.8850 | 59222.9164 | 8.480 | 0.039 | 17 | Ak2 | $I_C$ |
| 59223.0302 | 59223.0557 | 8.617 | 0.033 | 36 | Aka | $R_C$ |
| 59223.8821 | 59224.0308 | 8.703 | 0.035 | 212 | Aka | $R_C$ |
| 59223.8857 | 59223.9328 | 8.726 | 0.028 | 20 | Ak2 | $B$ |
| 59223.8863 | 59223.9335 | 8.726 | 0.036 | 20 | Ak2 | $V$ |
| 59223.8871 | 59223.9343 | 8.563 | 0.037 | 16 | Ak2 | $I_C$ |
| 59224.8688 | 59225.0565 | 8.770 | 0.033 | 295 | Aka | $R_C$ |
| 59224.8735 | 59224.8912 | 8.777 | 0.014 | 10 | Ak2 | $B$ |
| 59224.8742 | 59224.8918 | 8.780 | 0.013 | 10 | Ak2 | $V$ |
| 59224.8749 | 59224.8926 | 8.595 | 0.016 | 10 | Ak2 | $I_C$ |
| 59225.1965 | 59225.2445 | 8.771 | 0.029 | 140 | Kai | $R_C$ |
| 59226.1966 | 59226.2362 | 8.903 | 0.029 | 116 | Kai | $R_C$ |
| 59226.8834 | 59227.0325 | 9.092 | 0.045 | 269 | Aka | $R_C$ |
| 59226.8858 | 59226.9015 | 9.152 | 0.017 | 9 | Ak2 | $B$ |

**Table E1.** Log of observations of SS Cyg after BJD 2458700. (continued).

| Start* | End* | Mag† | Error‡ | $N$§ | Obs‖ | Band |
|---|---|---|---|---|---|---|
| 59226.8865 | 59226.9021 | 9.139 | 0.014 | 9 | Ak2 | $V$ |
| 59226.8873 | 59226.9029 | 8.902 | 0.013 | 9 | Ak2 | $I_C$ |
| 59227.8737 | 59228.0385 | 9.253 | 0.059 | 297 | Aka | $R_C$ |
| 59227.8766 | 59227.8962 | 9.327 | 0.033 | 11 | Ak2 | $B$ |
| 59227.8772 | 59227.8968 | 9.309 | 0.030 | 11 | Ak2 | $V$ |
| 59227.8780 | 59227.8976 | 9.017 | 0.032 | 11 | Ak2 | $I_C$ |
| 59228.8744 | 59229.0174 | 9.463 | 0.069 | 258 | Aka | $R_C$ |
| 59228.8798 | 59228.9033 | 9.576 | 0.051 | 12 | Ak2 | $B$ |
| 59228.8804 | 59228.9039 | 9.531 | 0.057 | 13 | Ak2 | $V$ |
| 59228.8812 | 59228.9028 | 9.241 | 0.059 | 12 | Ak2 | $I_C$ |
| 59230.8716 | 59230.9912 | 9.600 | 0.068 | 204 | Aka | $R_C$ |
| 59230.8736 | 59230.8952 | 9.813 | 0.055 | 12 | Ak2 | $B$ |
| 59230.8742 | 59230.8958 | 9.713 | 0.037 | 12 | Ak2 | $V$ |
| 59230.8750 | 59230.8966 | 9.300 | 0.042 | 13 | Ak2 | $I_C$ |
| 59231.8728 | 59231.9159 | 10.016 | 0.115 | 17 | Ak2 | $B$ |
| 59231.8735 | 59231.9166 | 9.902 | 0.112 | 17 | Ak2 | $V$ |
| 59231.8743 | 59231.9174 | 9.465 | 0.068 | 18 | Ak2 | $I_C$ |
| 59231.8854 | 59232.0174 | 9.819 | 0.080 | 223 | Aka | $R_C$ |
| 59233.8837 | 59233.9937 | 9.978 | 0.126 | 189 | Aka | $R_C$ |
| 59233.8851 | 59233.9067 | 10.394 | 0.166 | 12 | Ak2 | $B$ |
| 59233.8857 | 59233.9073 | 10.233 | 0.129 | 12 | Ak2 | $V$ |
| 59233.8865 | 59233.9081 | 9.658 | 0.114 | 12 | Ak2 | $I_C$ |
| 59234.8712 | 59234.8888 | 10.452 | 0.077 | 10 | Ak2 | $V$ |
| 59234.8739 | 59234.8896 | 9.815 | 0.054 | 9 | Ak2 | $I_C$ |
| 59234.8744 | 59234.8882 | 10.600 | 0.085 | 7 | Ak2 | $B$ |
| 59234.8749 | 59234.9839 | 10.175 | 0.073 | 197 | Aka | $R_C$ |
| 59235.8760 | 59235.8780 | 10.501 | 0.039 | 2 | Ak2 | $V$ |
| 59235.8785 | 59235.8946 | 10.282 | 0.065 | 23 | Aka | $R_C$ |
| 59238.9235 | 59238.9613 | 10.190 | 0.082 | 69 | Aka | $R_C$ |
| 59238.9305 | 59238.9579 | 10.431 | 0.131 | 15 | Ak2 | $V$ |
| 59238.9313 | 59238.9587 | 9.806 | 0.081 | 15 | Ak2 | $I_C$ |
| 59238.9318 | 59238.9592 | 10.661 | 0.144 | 15 | Ak2 | $B$ |
| 59239.8820 | 59239.9932 | 10.312 | 0.109 | 203 | Aka | $R_C$ |
| 59239.8867 | 59239.9043 | 10.602 | 0.084 | 10 | Ak2 | $V$ |
| 59239.8875 | 59239.9051 | 9.867 | 0.060 | 10 | Ak2 | $I_C$ |
| 59239.8880 | 59239.9057 | 10.925 | 0.116 | 10 | Ak2 | $B$ |
| 59241.8840 | 59241.9016 | 10.806 | 0.084 | 10 | Ak2 | $V$ |
| 59241.8853 | 59241.9030 | 11.134 | 0.113 | 10 | Ak2 | $B$ |
| 59241.8868 | 59241.9024 | 10.027 | 0.048 | 9 | Ak2 | $I_C$ |
| 59241.8888 | 59241.9823 | 10.497 | 0.109 | 168 | Aka | $R_C$ |
| 59242.8801 | 59242.8978 | 9.737 | 0.144 | 11 | Ak2 | $I_C$ |
| 59242.8813 | 59242.8970 | 10.385 | 0.262 | 7 | Ak2 | $V$ |
| 59242.8823 | 59242.9684 | 10.219 | 0.149 | 148 | Aka | $R_C$ |
| 59242.8826 | 59242.8963 | 10.605 | 0.243 | 8 | Ak2 | $B$ |
| 59243.8798 | 59243.8974 | 10.714 | 0.081 | 10 | Ak2 | $V$ |
| 59243.8806 | 59243.8982 | 9.900 | 0.085 | 10 | Ak2 | $I_C$ |
| 59243.8811 | 59243.8988 | 11.072 | 0.131 | 10 | Ak2 | $B$ |
| 59243.8820 | 59244.0066 | 10.409 | 0.120 | 225 | Aka | $R_C$ |
| 59244.8869 | 59244.9648 | 10.007 | 0.113 | 34 | Aka | $R_C$ |
| 59245.8818 | 59245.9939 | 9.426 | 0.070 | 193 | Aka | $R_C$ |
| 59245.8883 | 59245.9158 | 9.520 | 0.037 | 15 | Ak2 | $V$ |

**Table E1.** Log of observations of SS Cyg after BJD 2458700. (continued).

| Start* | End* | Mag† | Error‡ | $N$§ | Obs‖ | Band |
|---|---|---|---|---|---|---|
| 59245.8891 | 59245.9166 | 9.213 | 0.026 | 15 | Ak2 | $I_C$ |
| 59245.8896 | 59245.9151 | 9.602 | 0.054 | 14 | Ak2 | $B$ |
| 59247.8838 | 59247.9850 | 9.280 | 0.041 | 175 | Aka | $R_C$ |
| 59247.8878 | 59247.9114 | 9.355 | 0.033 | 13 | Ak2 | $V$ |
| 59247.8886 | 59247.9121 | 9.101 | 0.042 | 13 | Ak2 | $I_C$ |
| 59247.8892 | 59247.9127 | 9.385 | 0.040 | 13 | Ak2 | $B$ |
| 59248.8857 | 59248.9190 | 9.605 | 0.041 | 14 | Ak2 | $V$ |
| 59248.8865 | 59248.9198 | 9.289 | 0.041 | 16 | Ak2 | $I_C$ |
| 59248.8870 | 59248.9183 | 9.626 | 0.045 | 15 | Ak2 | $B$ |
| 59248.8882 | 59248.9845 | 9.506 | 0.047 | 96 | Aka | $R_C$ |
| 59249.8860 | 59249.9036 | 9.876 | 0.050 | 10 | Ak2 | $V$ |
| 59249.8868 | 59249.9044 | 9.498 | 0.053 | 10 | Ak2 | $I_C$ |
| 59249.8873 | 59249.9029 | 9.929 | 0.053 | 9 | Ak2 | $B$ |
| 59249.8878 | 59249.9956 | 9.784 | 0.047 | 195 | Aka | $R_C$ |
| 59251.8820 | 59251.9055 | 9.961 | 0.055 | 13 | Ak2 | $V$ |
| 59251.8833 | 59251.9049 | 10.061 | 0.053 | 12 | Ak2 | $B$ |
| 59251.8848 | 59251.9063 | 9.491 | 0.056 | 12 | Ak2 | $I_C$ |
| 59251.8850 | 59251.9116 | 9.787 | 0.060 | 49 | Aka | $R_C$ |
| 59252.8843 | 59252.9503 | 9.747 | 0.057 | 120 | Aka | $R_C$ |
| 59252.8878 | 59252.9113 | 9.864 | 0.057 | 13 | Ak2 | $V$ |
| 59252.8886 | 59252.9121 | 9.417 | 0.040 | 13 | Ak2 | $I_C$ |
| 59252.8891 | 59252.9107 | 9.987 | 0.082 | 11 | Ak2 | $B$ |
| 59253.9328 | 59253.9839 | 9.713 | 0.045 | 86 | Aka | $R_C$ |
| 59254.8927 | 59255.3840 | 9.827 | 0.080 | 75 | Aka | $R_C$ |
| 59254.8947 | 59254.9535 | 10.018 | 0.097 | 4 | Ak2 | $V$ |
| 59254.8955 | 59254.9700 | 9.569 | 0.085 | 10 | Ak2 | $I_C$ |
| 59254.8960 | 59254.9195 | 10.130 | 0.072 | 4 | Ak2 | $B$ |
| 59255.8903 | 59256.3820 | 9.755 | 0.109 | 131 | Aka | $R_C$ |
| 59255.8954 | 59255.9169 | 9.979 | 0.062 | 12 | Ak2 | $V$ |
| 59255.8962 | 59255.9177 | 9.461 | 0.049 | 12 | Ak2 | $I_C$ |
| 59255.8967 | 59255.9182 | 10.168 | 0.103 | 11 | Ak2 | $B$ |
| 59257.2244 | 59257.2716 | 9.894 | 0.066 | 134 | Kai | $R_C$ |
| 59257.8866 | 59258.3802 | 10.007 | 0.157 | 105 | Aka | $R_C$ |
| 59257.8887 | 59257.9102 | 9.604 | 0.090 | 12 | Ak2 | $I_C$ |
| 59257.8892 | 59257.9107 | 10.330 | 0.143 | 14 | Ak2 | $B$ |
| 59257.8899 | 59257.9114 | 10.159 | 0.101 | 12 | Ak2 | $V$ |
| 59259.3556 | 59259.3795 | 10.118 | 0.079 | 38 | Aka | $R_C$ |
| 59260.8898 | 59261.3713 | 9.540 | 0.054 | 68 | Aka | $R_C$ |
| 59261.9321 | 59261.9437 | 9.437 | 0.048 | 22 | Aka | $R_C$ |
| 59262.2404 | 59262.2613 | 9.480 | 0.041 | 52 | Kai | $R_C$ |
| 59262.9016 | 59263.3776 | 9.404 | 0.068 | 94 | Aka | $R_C$ |
| 59262.9174 | 59262.9199 | 9.165 | 0.057 | 3 | Ak2 | $I_C$ |
| 59263.2299 | 59263.2641 | 9.512 | 0.047 | 201 | Kai | $R_C$ |
| 59263.8902 | 59263.9020 | 9.572 | 0.056 | 7 | Ak2 | $V$ |
| 59263.8930 | 59263.9028 | 9.236 | 0.080 | 6 | Ak2 | $I_C$ |
| 59263.8935 | 59263.9033 | 9.687 | 0.042 | 5 | Ak2 | $B$ |
| 59263.8980 | 59263.9572 | 9.406 | 0.046 | 106 | Aka | $R_C$ |
| 59264.8949 | 59264.9145 | 9.744 | 0.049 | 11 | Ak2 | $V$ |
| 59264.8955 | 59265.3722 | 9.642 | 0.067 | 103 | Aka | $R_C$ |
| 59264.8957 | 59264.9153 | 9.384 | 0.057 | 11 | Ak2 | $I_C$ |
| 59264.8962 | 59264.9119 | 9.855 | 0.071 | 9 | Ak2 | $B$ |

**Table E1.** Log of observations of SS Cyg after BJD 2458700. (continued).

| Start* | End* | Mag† | Error‡ | $N$§ | Obs‖ | Band |
|---|---|---|---|---|---|---|
| 59265.2325 | 59265.2650 | 9.662 | 0.055 | 188 | Kai | $R_C$ |
| 59265.8985 | 59266.3793 | 9.886 | 0.062 | 94 | Aka | $R_C$ |
| 59265.8999 | 59265.9156 | 9.634 | 0.062 | 9 | Ak2 | $I_C$ |
| 59266.2315 | 59266.2601 | 9.791 | 0.044 | 168 | Kai | $R_C$ |
| 59266.8979 | 59267.3765 | 9.824 | 0.075 | 157 | Aka | $R_C$ |
| 59266.8991 | 59266.9148 | 9.995 | 0.055 | 9 | Ak2 | $V$ |
| 59266.8999 | 59266.9215 | 9.515 | 0.069 | 12 | Ak2 | $I_C$ |
| 59267.2300 | 59267.2636 | 9.870 | 0.075 | 197 | Kai | $R_C$ |
| 59267.9024 | 59267.9200 | 9.594 | 0.081 | 10 | Ak2 | $I_C$ |
| 59267.9030 | 59268.3734 | 9.939 | 0.082 | 121 | Aka | $R_C$ |
| 59268.2356 | 59268.2630 | 9.947 | 0.074 | 243 | Kai | $R_C$ |
| 59269.2361 | 59269.2620 | 10.025 | 0.060 | 229 | Kai | $R_C$ |
| 59269.3374 | 59269.3730 | 9.821 | 0.092 | 65 | Aka | $R_C$ |
| 59270.2363 | 59270.2593 | 9.760 | 0.084 | 200 | Kai | $R_C$ |
| 59270.3366 | 59270.3745 | 9.671 | 0.101 | 69 | Aka | $R_C$ |
| 59271.2330 | 59271.2564 | 9.845 | 0.098 | 205 | Kai | $R_C$ |
| 59273.2352 | 59273.2515 | 10.103 | 0.091 | 211 | Kai | $R_C$ |
| 59273.9014 | 59274.3743 | 10.119 | 0.104 | 78 | Aka | $R_C$ |
| 59273.9075 | 59273.9173 | 9.817 | 0.119 | 2 | Ak2 | $I_C$ |
| 59274.2378 | 59274.2479 | 10.049 | 0.085 | 130 | Kai | $R_C$ |
| 59275.2348 | 59275.2467 | 9.954 | 0.110 | 146 | Kai | $R_C$ |
| 59275.6297 | 59275.6917 | 10.035 | 0.119 | 326 | TRT | $V$ |
| 59275.9118 | 59276.3670 | 9.878 | 0.106 | 109 | Aka | $R_C$ |
| 59276.2339 | 59276.2436 | 9.951 | 0.087 | 134 | Kai | $R_C$ |
| 59277.3207 | 59277.3657 | 9.912 | 0.068 | 82 | Aka | $R_C$ |
| 59279.6355 | 59279.6776 | 9.870 | 0.073 | 276 | TRT | $V$ |
| 59280.2940 | 59280.3649 | 9.479 | 0.062 | 129 | Aka | $R_C$ |
| 59280.3343 | 59280.3637 | 9.603 | 0.027 | 16 | Ak2 | $V$ |
| 59280.3348 | 59280.3642 | 9.460 | 0.040 | 16 | Ak2 | $R_C$ |
| 59280.3351 | 59280.3646 | 9.291 | 0.037 | 16 | Ak2 | $I_C$ |
| 59280.3357 | 59280.3631 | 9.662 | 0.058 | 15 | Ak2 | $B$ |
| 59281.5606 | 59281.6634 | 9.276 | 0.054 | 59 | Vih | $R_C$ |
| 59281.5611 | 59281.6639 | 9.109 | 0.055 | 59 | Vih | $I_C$ |
| 59281.5617 | 59281.6645 | 9.424 | 0.061 | 60 | Vih | $V$ |
| 59282.2955 | 59282.3572 | 9.445 | 0.068 | 90 | Aka | $R_C$ |
| 59282.3304 | 59282.3579 | 9.577 | 0.057 | 15 | Ak2 | $V$ |
| 59282.3309 | 59282.3584 | 9.423 | 0.056 | 15 | Ak2 | $R_C$ |
| 59282.3312 | 59282.3469 | 9.267 | 0.051 | 9 | Ak2 | $I_C$ |
| 59282.3317 | 59282.3415 | 9.667 | 0.062 | 6 | Ak2 | $B$ |
| 59282.5834 | 59282.6654 | 9.595 | 0.051 | 60 | Vih | $V$ |
| 59282.5845 | 59282.6663 | 9.245 | 0.051 | 60 | Vih | $I_C$ |
| 59282.5877 | 59282.6604 | 9.421 | 0.053 | 54 | Vih | $R_C$ |
| 59283.3121 | 59283.3638 | 9.633 | 0.076 | 94 | Aka | $R_C$ |
| 59283.3208 | 59283.3658 | 9.624 | 0.074 | 24 | Ak2 | $R_C$ |
| 59283.3223 | 59283.3654 | 9.831 | 0.107 | 23 | Ak2 | $V$ |
| 59283.3250 | 59283.3622 | 9.417 | 0.071 | 20 | Ak2 | $I_C$ |
| 59283.3314 | 59283.3549 | 9.938 | 0.093 | 13 | Ak2 | $B$ |
| 59284.2932 | 59284.3622 | 9.835 | 0.051 | 125 | Aka | $R_C$ |
| 59284.3207 | 59284.3621 | 10.015 | 0.062 | 22 | Ak2 | $V$ |
| 59284.3212 | 59284.3626 | 9.798 | 0.068 | 22 | Ak2 | $R_C$ |
| 59284.3215 | 59284.3629 | 9.540 | 0.066 | 22 | Ak2 | $I_C$ |

**Table E1.** Log of observations of SS Cyg after BJD 2458700. (continued).

| Start* | End* | Mag† | Error‡ | $N$§ | Obs‖ | Band |
|---|---|---|---|---|---|---|
| 59284.3220 | 59284.3614 | 10.120 | 0.065 | 21 | Ak2 | $B$ |
| 59284.6081 | 59284.6715 | 10.040 | 0.051 | 429 | TRT | $V$ |
| 59284.6534 | 59284.6758 | 10.057 | 0.086 | 15 | Vih | $V$ |
| 59284.6556 | 59284.6699 | 9.803 | 0.067 | 10 | Vih | $R_C$ |
| 59284.6575 | 59284.6719 | 9.583 | 0.045 | 10 | Vih | $I_C$ |
| 59286.6076 | 59286.6797 | 10.324 | 0.087 | 498 | TRT | $V$ |
| 59286.9315 | 59286.9346 | 10.571 | 0.034 | 4 | HBB | $V$ |
| 59286.9321 | 59286.9351 | 10.879 | 0.035 | 4 | HBB | $B$ |
| 59287.2786 | 59287.3582 | 10.207 | 0.059 | 144 | Aka | $R_C$ |
| 59287.3098 | 59287.3590 | 10.151 | 0.047 | 26 | Ak2 | $R_C$ |
| 59287.3133 | 59287.3586 | 10.439 | 0.052 | 24 | Ak2 | $V$ |
| 59287.3141 | 59287.3574 | 9.834 | 0.047 | 23 | Ak2 | $I_C$ |
| 59287.3244 | 59287.3520 | 10.601 | 0.071 | 15 | Ak2 | $B$ |
| 59288.2809 | 59288.3576 | 10.008 | 0.143 | 139 | Aka | $R_C$ |
| 59288.3196 | 59288.3548 | 10.394 | 0.051 | 19 | Ak2 | $V$ |
| 59288.3200 | 59288.3592 | 10.065 | 0.062 | 21 | Ak2 | $R_C$ |
| 59288.3223 | 59288.3537 | 9.757 | 0.049 | 17 | Ak2 | $I_C$ |
| 59289.3129 | 59289.3146 | 10.205 | 0.161 | 4 | Aka | $R_C$ |
| 59290.2999 | 59290.3572 | 10.411 | 0.085 | 104 | Aka | $R_C$ |
| 59291.2851 | 59291.3557 | 10.393 | 0.132 | 128 | Aka | $R_C$ |
| 59291.3058 | 59291.3548 | 10.719 | 0.154 | 26 | Ak2 | $V$ |
| 59291.3063 | 59291.3553 | 10.376 | 0.130 | 26 | Ak2 | $R_C$ |
| 59291.3067 | 59291.3537 | 9.990 | 0.109 | 25 | Ak2 | $I_C$ |
| 59291.3072 | 59291.3483 | 10.930 | 0.191 | 22 | Ak2 | $B$ |
| 59291.9038 | 59291.9355 | 10.477 | 0.138 | 22 | HBB | $V$ |
| 59291.9044 | 59291.9360 | 10.762 | 0.164 | 22 | HBB | $B$ |
| 59292.2989 | 59292.3557 | 10.197 | 0.099 | 103 | Aka | $R_C$ |
| 59292.3142 | 59292.3554 | 10.455 | 0.120 | 18 | Ak2 | $V$ |
| 59292.3147 | 59292.3558 | 10.156 | 0.098 | 19 | Ak2 | $R_C$ |
| 59292.3150 | 59292.3542 | 9.826 | 0.087 | 16 | Ak2 | $I_C$ |
| 59292.3155 | 59292.3449 | 10.684 | 0.136 | 13 | Ak2 | $B$ |
| 59293.2713 | 59293.3537 | 10.306 | 0.074 | 149 | Aka | $R_C$ |
| 59293.3039 | 59293.3529 | 10.555 | 0.096 | 26 | Ak2 | $V$ |
| 59293.3043 | 59293.3554 | 10.251 | 0.079 | 27 | Ak2 | $R_C$ |
| 59293.3047 | 59293.3478 | 9.909 | 0.073 | 23 | Ak2 | $I_C$ |
| 59293.3071 | 59293.3425 | 10.594 | 0.120 | 4 | Ak2 | $B$ |
| 59293.5410 | 59293.6183 | 10.667 | 0.081 | 167 | Vih | $R_C$ |
| 59294.5406 | 59294.6433 | 10.300 | 0.087 | 225 | Vih | $R_C$ |
| 59295.2904 | 59295.3526 | 10.285 | 0.066 | 113 | Aka | $R_C$ |
| 59295.3049 | 59295.3500 | 10.551 | 0.079 | 24 | Ak2 | $V$ |
| 59295.3054 | 59295.3505 | 10.256 | 0.057 | 24 | Ak2 | $R_C$ |
| 59295.3057 | 59295.3508 | 9.937 | 0.053 | 24 | Ak2 | $I_C$ |
| 59295.3063 | 59295.3494 | 10.752 | 0.088 | 23 | Ak2 | $B$ |
| 59296.2776 | 59296.3500 | 10.511 | 0.084 | 77 | Aka | $R_C$ |
| 59297.2728 | 59297.3524 | 10.287 | 0.071 | 144 | Aka | $R_C$ |
| 59298.5969 | 59298.6386 | 10.183 | 0.086 | 32 | Vih | $V$ |
| 59298.5973 | 59298.6390 | 9.945 | 0.068 | 32 | Vih | $R_C$ |
| 59298.5978 | 59298.6394 | 9.675 | 0.065 | 32 | Vih | $I_C$ |
| 59299.2569 | 59299.3481 | 10.131 | 0.115 | 165 | Aka | $R_C$ |
| 59300.2599 | 59300.3511 | 10.053 | 0.084 | 165 | Aka | $R_C$ |
| 59300.6294 | 59300.6417 | 10.184 | 0.084 | 10 | Vih | $V$ |

**Table E1.** Log of observations of SS Cyg after BJD 2458700. (continued).

| Start* | End* | Mag† | Error‡ | $N$§ | Obs‖ | Band |
|---|---|---|---|---|---|---|
| 59300.6299 | 59300.6422 | 9.949 | 0.064 | 10 | Vih | $R_C$ |
| 59300.6304 | 59300.6426 | 9.702 | 0.048 | 10 | Vih | $I_C$ |
| 59302.2437 | 59302.3299 | 10.048 | 0.083 | 156 | Aka | $R_C$ |
| 59302.5572 | 59302.5858 | 9.388 | 0.039 | 22 | Vih | $V$ |
| 59302.5576 | 59302.5863 | 9.267 | 0.036 | 22 | Vih | $R_C$ |
| 59302.5594 | 59302.5867 | 9.125 | 0.035 | 21 | Vih | $I_C$ |
| 59303.2798 | 59303.3466 | 9.241 | 0.049 | 121 | Aka | $R_C$ |
| 59304.3041 | 59304.3398 | 9.211 | 0.032 | 128 | Kty | $R_C$ |
| 59304.6104 | 59304.6766 | 9.235 | 0.043 | 432 | Kai | $R_C$ |
| 59305.2443 | 59305.3467 | 9.377 | 0.057 | 164 | Aka | $R_C$ |
| 59305.6113 | 59305.6756 | 9.405 | 0.041 | 368 | Kai | $R_C$ |
| 59306.2509 | 59306.3456 | 9.543 | 0.044 | 147 | Aka | $R_C$ |
| 59307.2654 | 59307.3077 | 9.846 | 0.038 | 28 | Aka | $R_C$ |
| 59307.6367 | 59307.6774 | 9.778 | 0.070 | 175 | Kai | $R_C$ |
| 59308.5986 | 59308.6747 | 10.009 | 0.081 | 422 | Kai | $R_C$ |
| 59309.4997 | 59309.5184 | 10.301 | 0.049 | 18 | Vih | $V$ |
| 59309.5003 | 59309.5180 | 9.780 | 0.049 | 16 | Vih | $I_C$ |
| 59309.5200 | 59309.6062 | 9.950 | 0.074 | 201 | Vih | $R_C$ |
| 59309.5712 | 59309.6056 | 10.201 | 0.069 | 81 | Vi1 | $V$ |
| 59311.5150 | 59311.6246 | 10.415 | 0.104 | 122 | Vih | $V$ |
| 59311.5164 | 59311.6251 | 10.141 | 0.078 | 121 | Vih | $R_C$ |
| 59315.4727 | 59315.6125 | 10.330 | 0.103 | 327 | Vih | $R_C$ |
| 59315.5134 | 59315.5835 | 10.621 | 0.140 | 165 | Vih | $V$ |
| 59326.8485 | 59326.9074 | 10.317 | 0.152 | 38 | HBB | $V$ |
| 59326.8490 | 59326.9079 | 10.646 | 0.194 | 38 | HBB | $B$ |
| 59349.8523 | 59349.8801 | 10.714 | 0.118 | 60 | HBB | $V$ |
| 59362.8096 | 59362.9062 | 10.170 | 0.048 | 94 | HBB | $V$ |
| 59362.8109 | 59362.9066 | 10.363 | 0.053 | 94 | HBB | $B$ |
| 59362.8113 | 59362.9069 | 9.959 | 0.045 | 94 | HBB | $R_C$ |
| 59376.8430 | 59376.8878 | 10.727 | 0.127 | 35 | HBB | $V$ |
| 59376.8435 | 59376.8870 | 11.123 | 0.171 | 34 | HBB | $B$ |
| 59376.8439 | 59376.8874 | 10.337 | 0.103 | 34 | HBB | $R_C$ |
| 59377.8327 | 59377.8907 | 10.948 | 0.144 | 44 | HBB | $V$ |
| 59377.8332 | 59377.8899 | 10.410 | 0.176 | 43 | HBB | $B$ |
| 59377.8336 | 59377.8903 | 11.487 | 0.109 | 43 | HBB | $R_C$ |
| 59378.8566 | 59378.8933 | 11.103 | 0.152 | 29 | HBB | $V$ |
| 59378.8571 | 59378.8925 | 11.556 | 0.199 | 28 | HBB | $B$ |
| 59378.8575 | 59378.8929 | 10.624 | 0.119 | 28 | HBB | $R_C$ |
| 59391.7347 | 59391.8605 | 9.074 | 0.066 | 120 | HBB | $V$ |
| 59391.7351 | 59391.8598 | 9.083 | 0.040 | 120 | HBB | $B$ |

*BJD − 2400000.0.

†Mean magnitude.

‡$1\sigma$ of mean magnitude.

§Number of observations.

‖Observer's code: Vih & Vi1 (Vihorlat Observatory), Ioh (Hiroshi Itoh), Kai (Kiyoshi Kasai), TRT (Tamás Tordai), CRI (Crimean Astrophysical Observatory), HBB (Franz-Josef Hambsch), Aka & Ak2 (Hidehiko Akazawa), Kty (Toshihiko Katayama).

**Table E2.** Log of observations in Event A and Event B in SS Cyg with *NICER*.

| NICER ObsID | Start* | End* | On-source time† | Average rate‡ |
|---|---|---|---|---|
| 3201600122 | 59011.4600 | 59011.4708 | 934 | 161 |
| 3201600136 | 59130.9386 | 59131.0157 | 2085 | 180 |
| 3201600137 | 59135.9719 | 59135.9972 | 2185 | 152 |
| 3201600138 | 59137.0043 | 59137.0218 | 1514 | 117 |
| 3201600139 | 59139.9092 | 59140.1684 | 450 | 207 |
| 3201600140 | 59142.9411 | 59143.0186 | 2286 | 218 |
| 3201600141 | 59143.9791 | 59144.0507 | 1225 | 188 |
| 3201600144 | 59162.9101 | 59162.9358 | 2213 | 181 |
| 3201600145 | 59166.9743 | 59167.0017 | 2373 | 213 |
| 3201600146 | 59168.0069 | 59168.0353 | 2450 | 144 |
| 3201600147 | 59170.9752 | 59171.0043 | 2511 | 132 |
| 3201600148 | 59171.9449 | 59171.9723 | 2371 | 172 |
| 3201600149 | 59173.9531 | 59173.9569 | 328 | 161 |
| 3201600150 | 59244.3413 | 59244.4113 | 930 | 294 |
| 3201600151 | 59244.5996 | 59244.8629 | 1270 | 291 |
| 3201600153 | 59269.3625 | 59269.4306 | 724 | 353 |
| 3201600154 | 59269.4903 | 59269.6888 | 1246 | 307 |
| 3201600155 | 59274.6043 | 59274.8722 | 4730 | 313 |
| 4201600101 | 59277.1067 | 59277.4354 | 1482 | 403 |
| 4201600102 | 59277.4939 | 59277.7583 | 1089 | 376 |
| 4201600103 | 59279.9463 | 59280.3404 | 2585 | 310 |

*BJD−2400000.0.

†Units of seconds.

‡NICER count rate in 0.3–7 keV in units of counts/sec.

**Table E3.** Log of observations in Event A and Event B in SS Cyg with *NuSTAR*.

| NuSTAR ObsID | Start* | End* | On-source time† | Average rate‡ |
|---|---|---|---|---|
| 90601329004 | 59130.6800 | 59131.1602 | 22970 | 14.5 |
| 90601329006 | 59135.5109 | 59136.0107 | 22930 | 13.2 |
| 90701304002 | 59244.3372 | 59244.9139 | 29430 | 22.6 |
| 90702309002 | 59274.4583 | 59274.8998 | 23500 | 30.8 |
| 90702309004 | 59279.8909 | 59280.3958 | 24800 | 30.5 |

*BJD−2400000.0.

†Units of seconds.

‡NuSTAR count rate in 3–79 keV in units of counts/sec.

**Table E4.** Results of the fitting of power spectra. Here, the errors are $1\sigma$ errors.

| Start* | End* | Duration† | $a$‡ | $b$§ | $c$¶ | Radius‖ |
|---|---|---|---|---|---|---|
| 59130.9386 | 59130.9502 | 1000 | 0.004±0.002 | 0.013±0.007 | 0.010±0.001 | $(2.7\pm1.0)\times10^9$ |
| 59135.9719 | 59135.9972 | 2185 | 0.004±0.001 | 0.008±0.003 | 0.013±0.001 | $(3.8\pm1.1)\times10^9$ |
| 59137.0043 | 59137.0218 | 1514 | 0.008±0.004 | 0.004±0.002 | 0.017±0.001 | $(6.2\pm2.2)\times10^9$ |
| 59142.9411 | 59142.9544 | 1153 | 0.003±0.001 | 0.018±0.007 | 0.011±0.001 | $(2.3\pm0.6)\times10^9$ |
| 59143.0055 | 59143.0186 | 1133 | 0.003±0.001 | 0.014±0.006 | 0.008±0.001 | $(2.4\pm0.7)\times10^9$ |
| 59144.0436 | 59144.0505 | 593 | 0.007±0.003 | 0.007±0.003 | 0.008±0.001 | $(4.0\pm1.2)\times10^9$ |
| 59162.9101 | 59162.9331 | 1984 | 0.003±0.001 | 0.016±0.005 | 0.012±0.001 | $(2.4\pm0.4)\times10^9$ |
| 59168.0069 | 59168.0314 | 2117 | 0.012±0.003 | 0.006±0.002 | 0.014±0.001 | $(4.7\pm0.9)\times10^9$ |
| 59170.9752 | 59171.0043 | 2511 | 0.006±0.002 | 0.007±0.002 | 0.014±0.001 | $(4.2\pm1.0)\times10^9$ |
| 59171.9449 | 59171.9723 | 2371 | 0.005±0.002 | 0.010±0.004 | 0.011± 0.001 | $(3.1\pm0.7)\times10^9$ |
| 59274.7978 | 59274.8077 | 861 | 0.005±0.001 | 0.027±0.008 | 0.013±0.001 | $(1.7\pm0.3)\times10^9$ |
| 59277.4939 | 59277.5001 | 533 | 0.002±0.001 | 0.031±0.012 | 0.004±0.001 | $(1.5\pm0.4)\times10^9$ |
| 59280.3376 | 59280.3403 | 243 | 0.003±0.001 | 0.028±0.014 | 0.009±0.001 | $(1.6\pm0.5)\times10^9$ |

*BJD−2400000.0.

†Units of seconds.

‡The estimated parameter in equation (3), which corresponds to the normalization.

§The estimated parameter in equation (3), which corresponds to the break frequency.

¶The estimated parameter in equation (3), which corresponds to the white noise.

‖The innermost disk radius in units of cm.

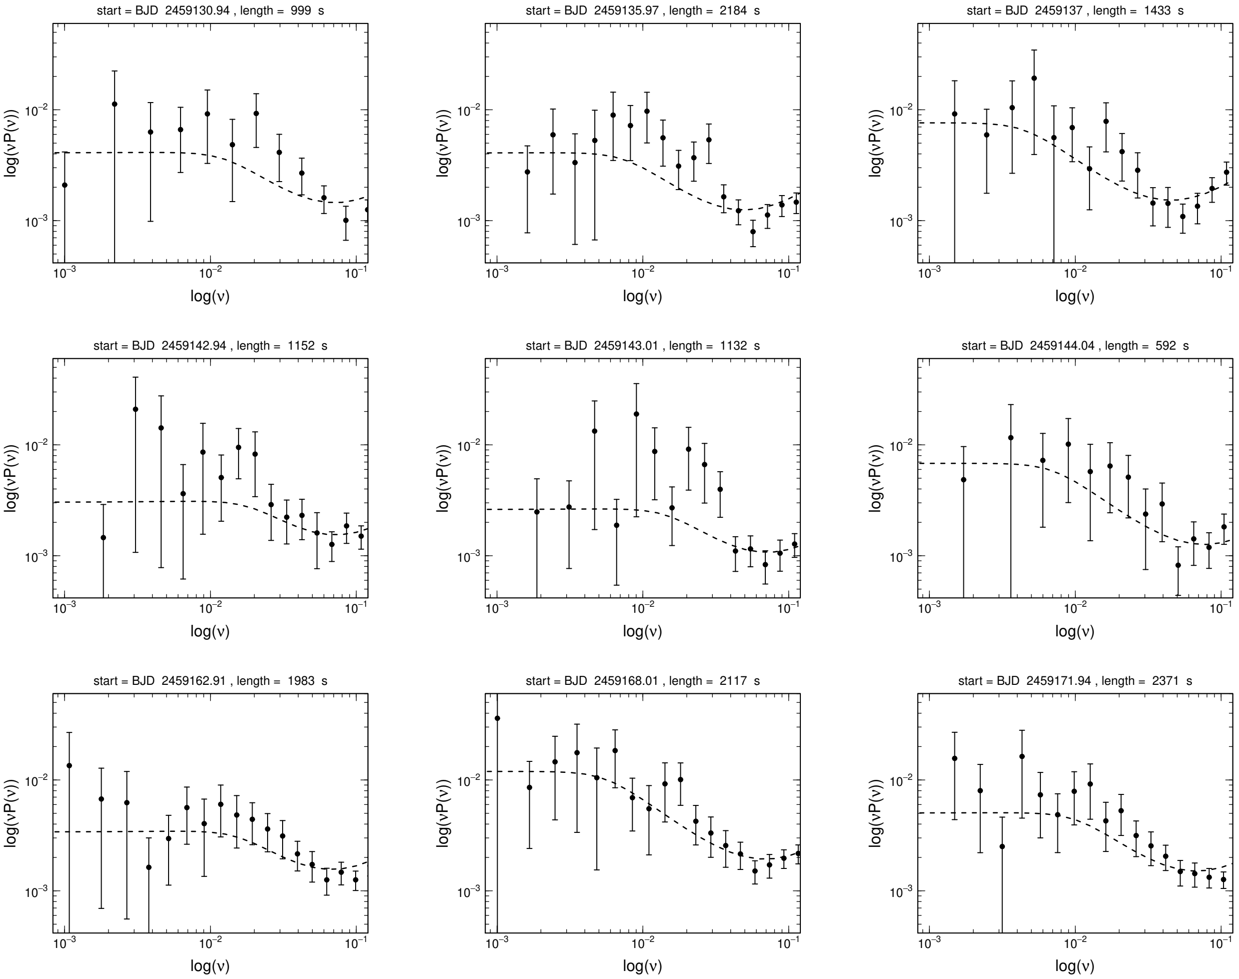


**Fig. E4.** Power spectra and fitting results of the *NICER* light curves during Event A. The black points and bars penetrating them represent the powers multiplied by the frequencies and their error bars. The dashed line stands for the result of our fitting. The start time of the observation and the length of the window are given at the top of each panel.

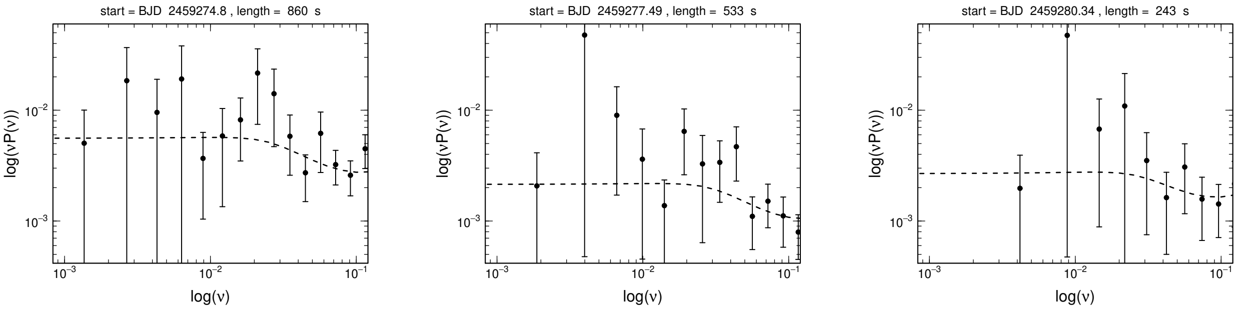


**Fig. E5.** Same as Fig. E3 but during Event B.

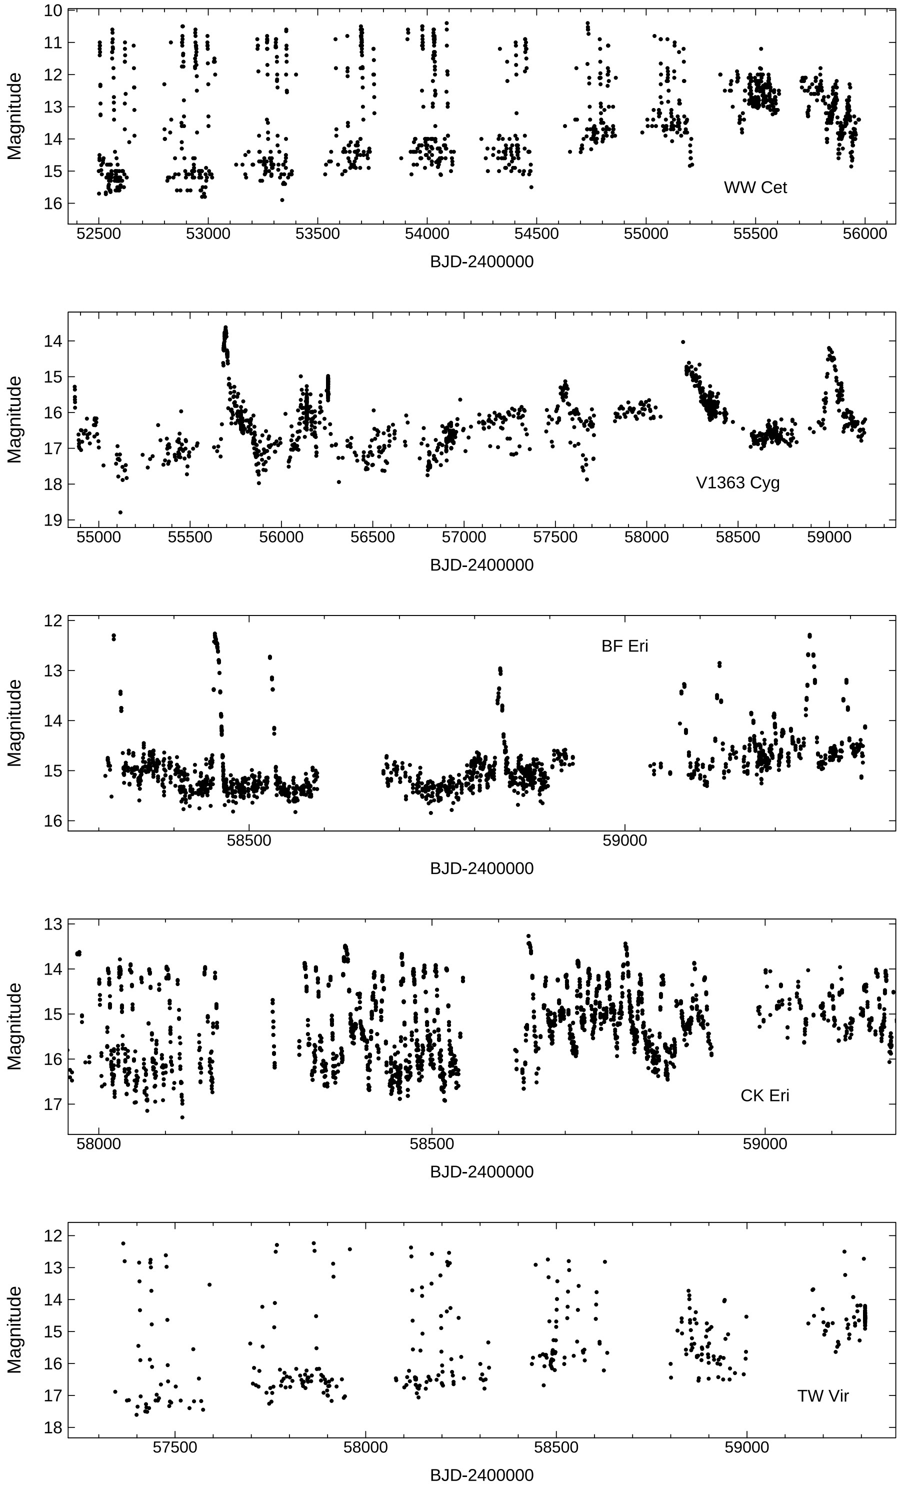


**Fig. E6.** Dwarf novae that have entered standstill or have exhibited gradual increases in the optical luminosity. The name of the object is given in each panel. The data are taken from the AAVSO archive and/or the ASAS-SN data archive and/or the Zwicky Transient Facility (ZTF; Bellm et al. 2019) public data.
